# Supplementary material for: Search for Dormant Black Holes in Ellipsoidal Variables III. The OGLE BULGE Short-Period Sample
Source: arXiv:2104.13221 ancillary file (2021-04-27)
Supplement: Supplementary file 1 [file BHIII_supplementary.pdf]

# Search for Dormant Black Holes in Ellipsoidal Variables III. The OGLE BULGE Short-Period Sample: supplemental document

Roy Gomel,<sup>1\*</sup> Simchon Faigler,<sup>1</sup> Tsevi Mazeh<sup>1</sup> and Michał Pawlak<sup>2</sup>

<sup>1</sup>*School of Physics and Astronomy, Tel Aviv University, Tel Aviv, 6997801, Israel*

<sup>2</sup>*Astronomical Observatory, Jagiellonian University, ul. Orla 171, 30-244 Kraków, Poland*

Accepted XXX. Received YYY; in original form ZZZ

**Key words:** methods: data analysis – techniques: photometric – binaries:  
close – stars: black holes

## 1 OGLE LIGHT CURVES OF OUR CANDIDATES

This section presents folded light curves in the OGLE *I* band of our 136 candidates. Each light curve was detrended by subtraction of the stellar averaged magnitude, fitted for each season separately, as described in the paper. For each system, the last six digits of the OGLE identifier are indicated together with the OGLE period [days] and the derived mMMR. A four-harmonics model is plotted with a solid line on top of the light curve. The residuals are plotted in the lower panels. The data (in both panels) are shown between the 1st–99th percentiles for clarity.

## 2 DATA TABLE OF OUR CANDIDATES

Given below a summary table containing results of the analysis performed on our 136 candidates. Each system parameters are given in two following lines: a first line with derived quantities and a second line with corresponding errors. The listed parameters are: OGLE ID (last six digits), OGLE orbital period [days], reference time [JD-2450000], reference-time

\* E-mail: roygomel@tauex.tau.ac.il

error, fitted I magnitude, fitted I magnitude error, cosine and sine Fourier coefficients, each followed by its error [mag], total number of analyzed points, total number of analyzed seasons, light-curve time range [days], reduced  $\chi^2$  of the four-harmonic model, mMMR and lower-percentile mMMR. Additional details are found in the paper, and the full table for all 10,956 short-period sample is available at the CDS.

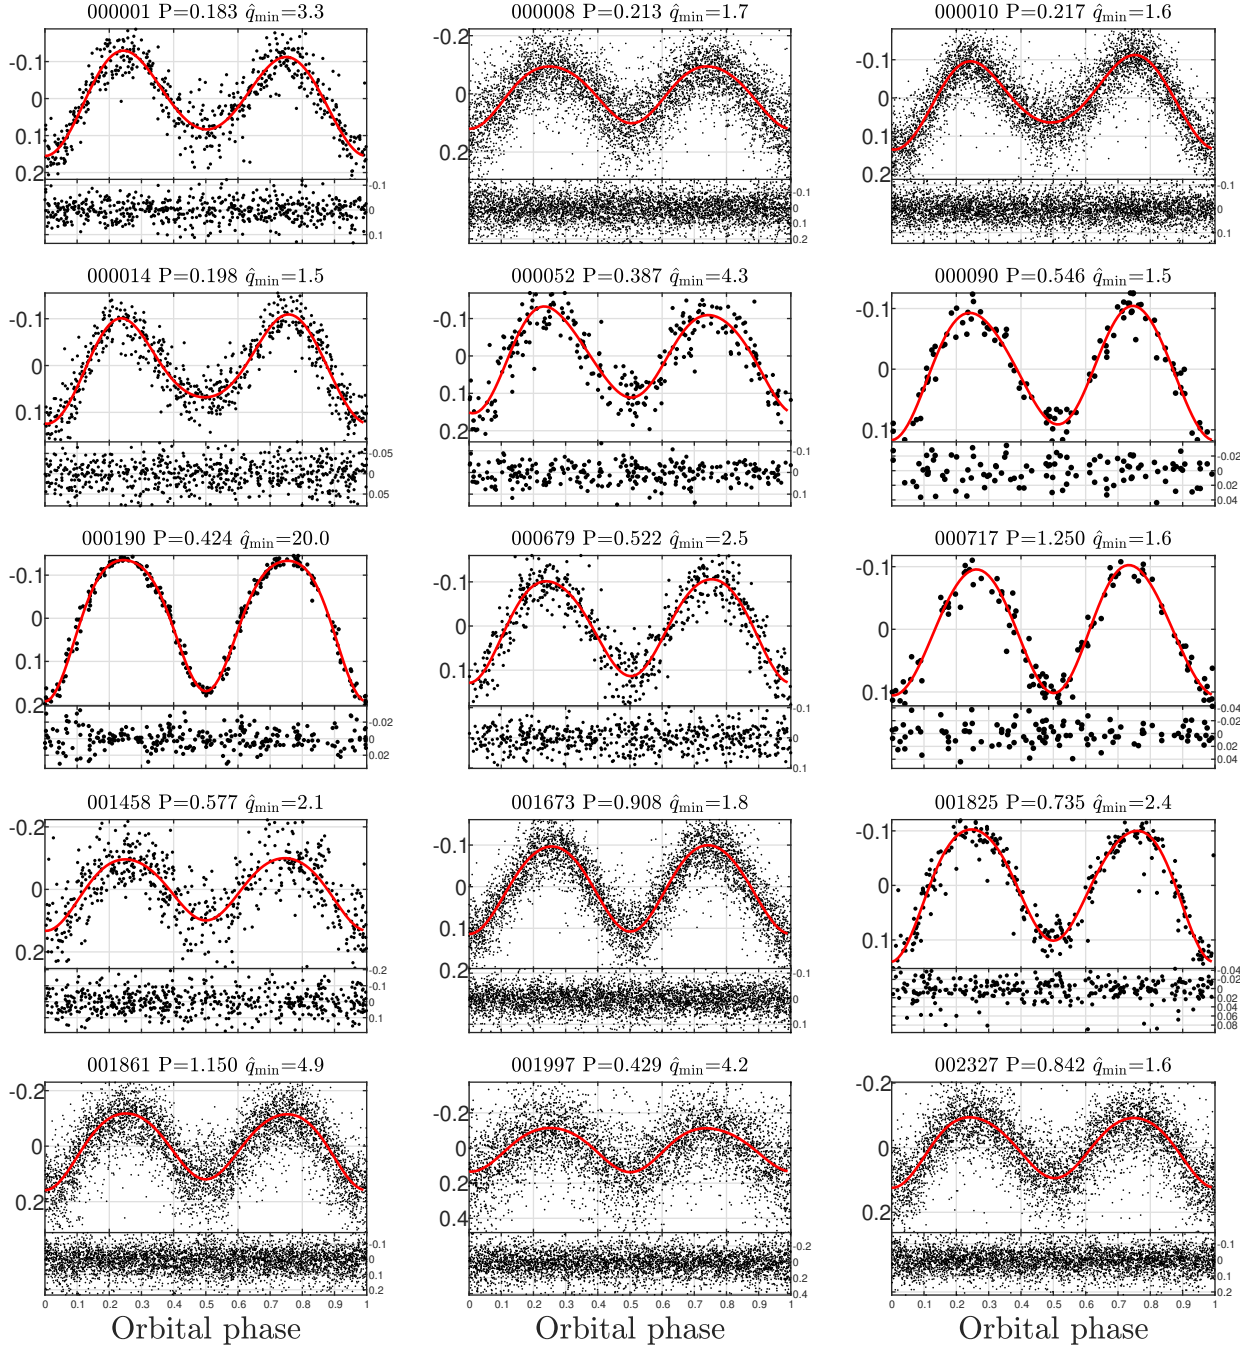

**Figure S1.** Folded detrended OGLE light curves in the *I* band of our 136 candidates. The last six digits of the OGLE identifier are indicated together with the OGLE period in days and  $\hat{q}_{\min}$ . Zero phase is defined at the epoch of the second-harmonic minimum. A four harmonics model is plotted with a solid line. The dominant  $A_2$  coefficient gives the characteristic double-peaked appearance to the light curve, while  $A_1$  and  $A_3$  are related to the difference between the minima. The residuals are plotted in the lower panels. The data (in both panels) are shown between the 1st–99th percentiles for clarity.

This paper has been typeset from a  $\text{\LaTeX}$  file prepared by the author.

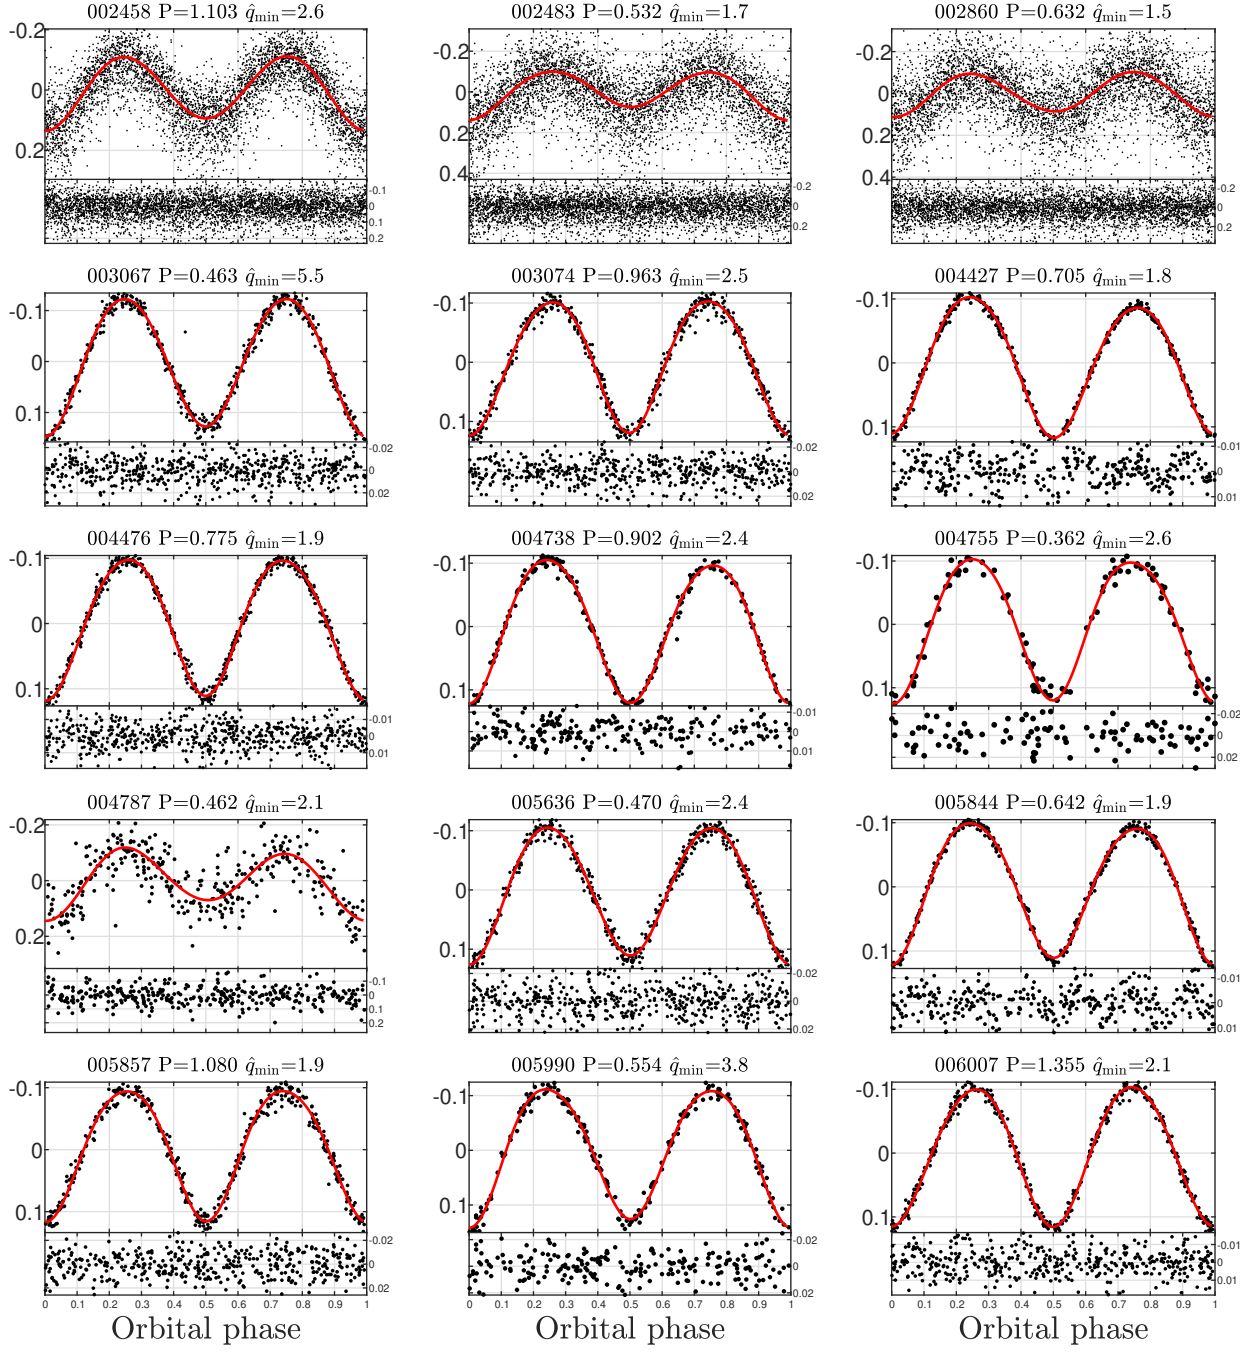

Figure S1. Continued



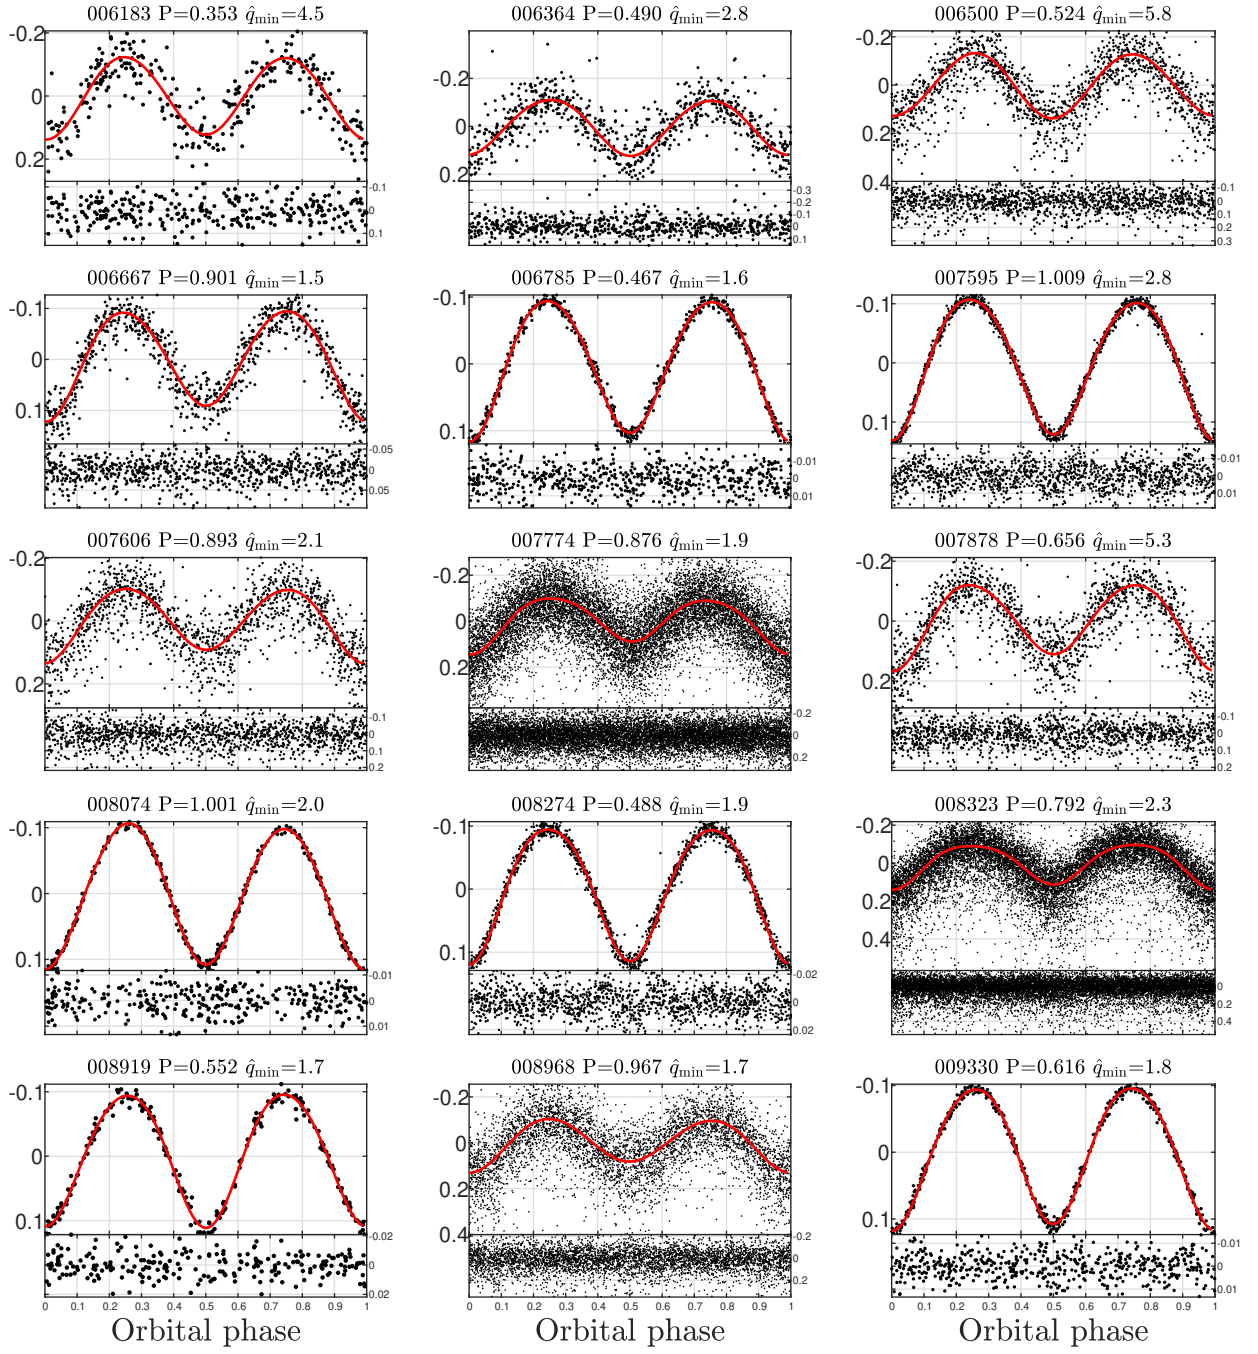

Figure S1. Continued

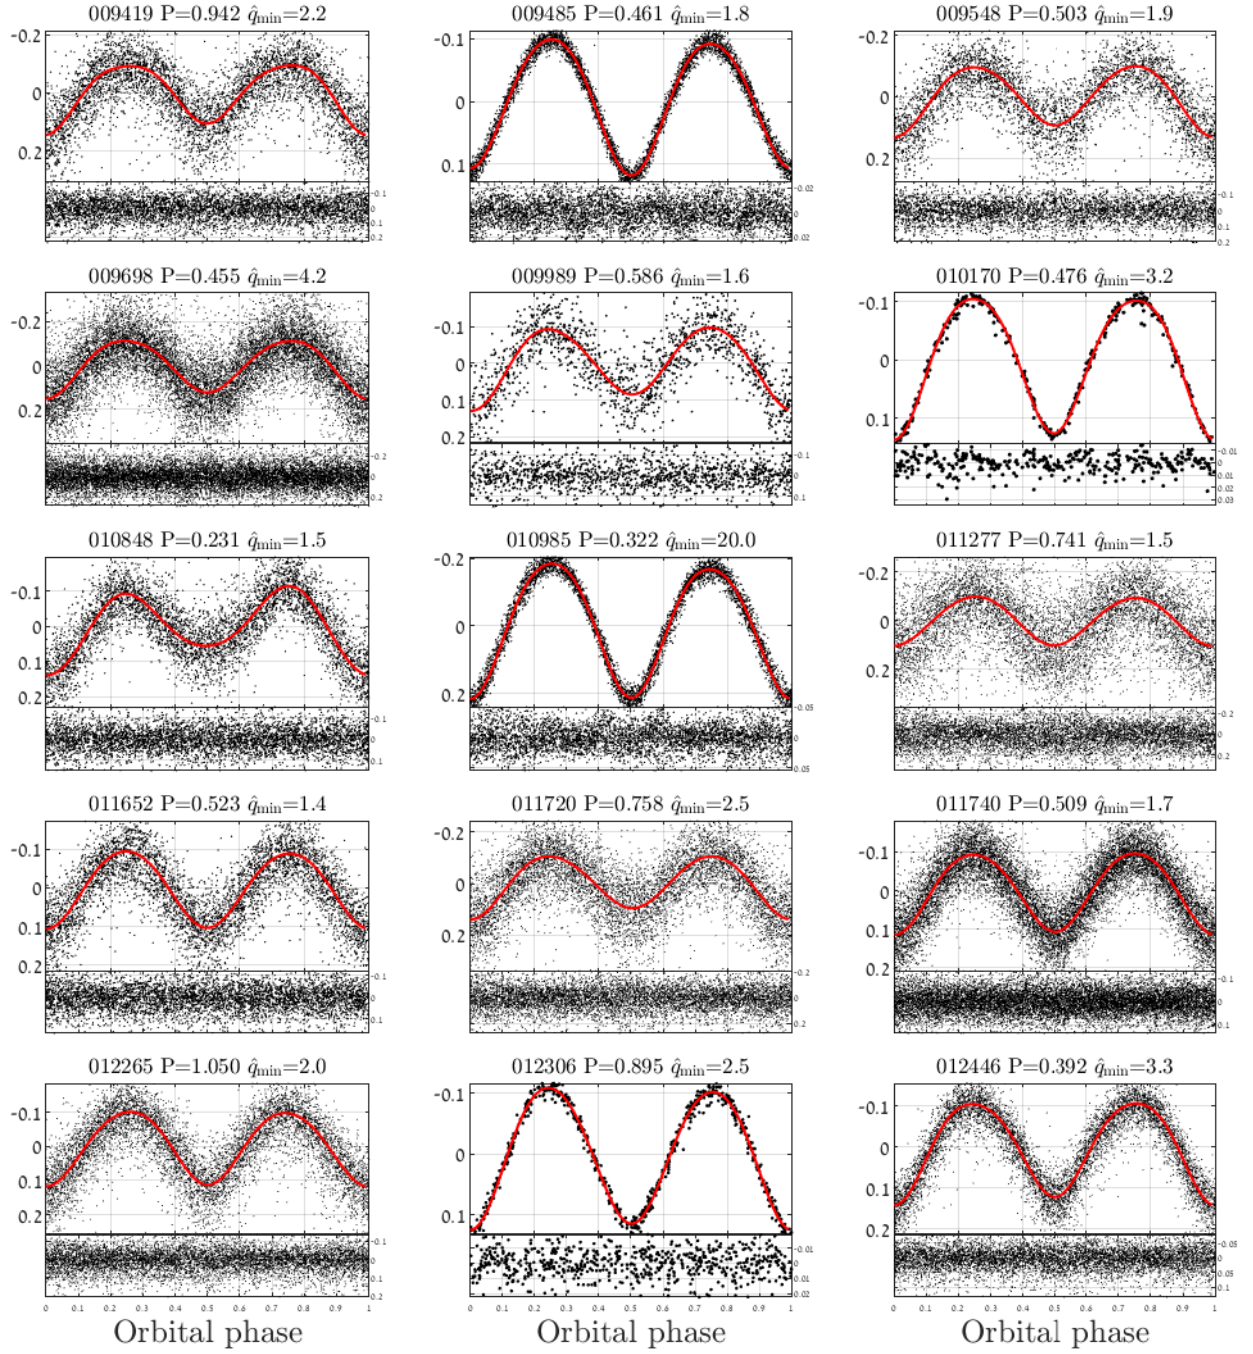

Figure S1. Continued



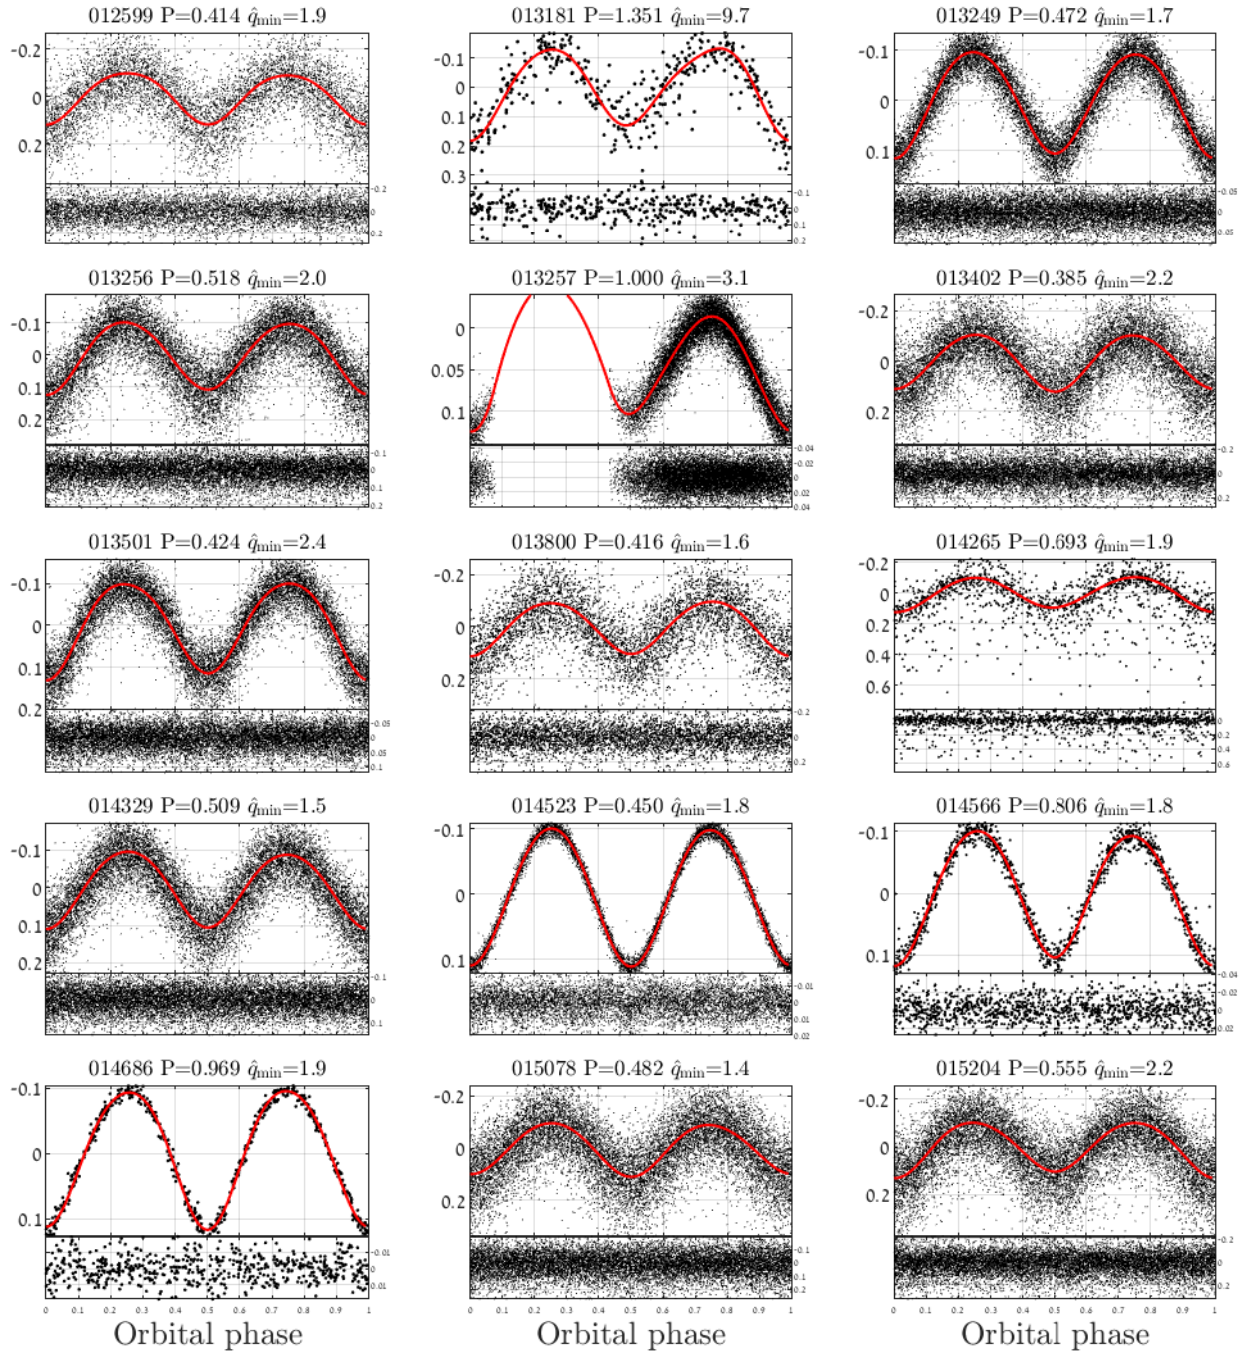

Figure S1. Continued

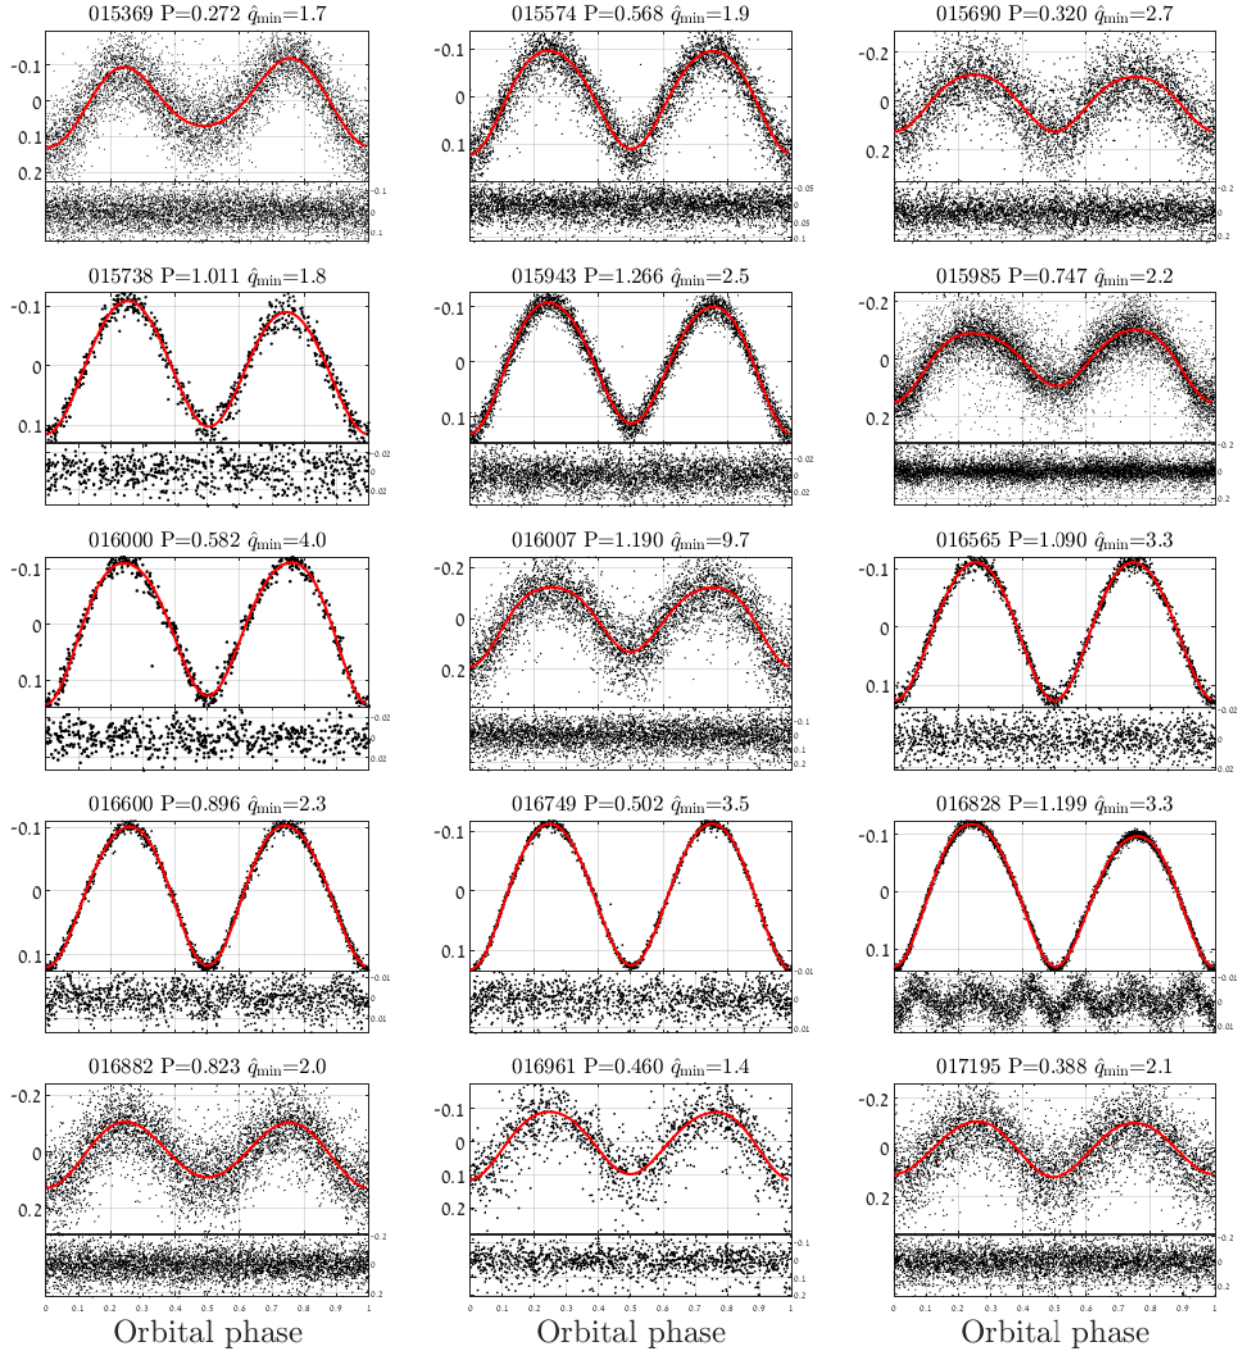

Figure S1. Continued



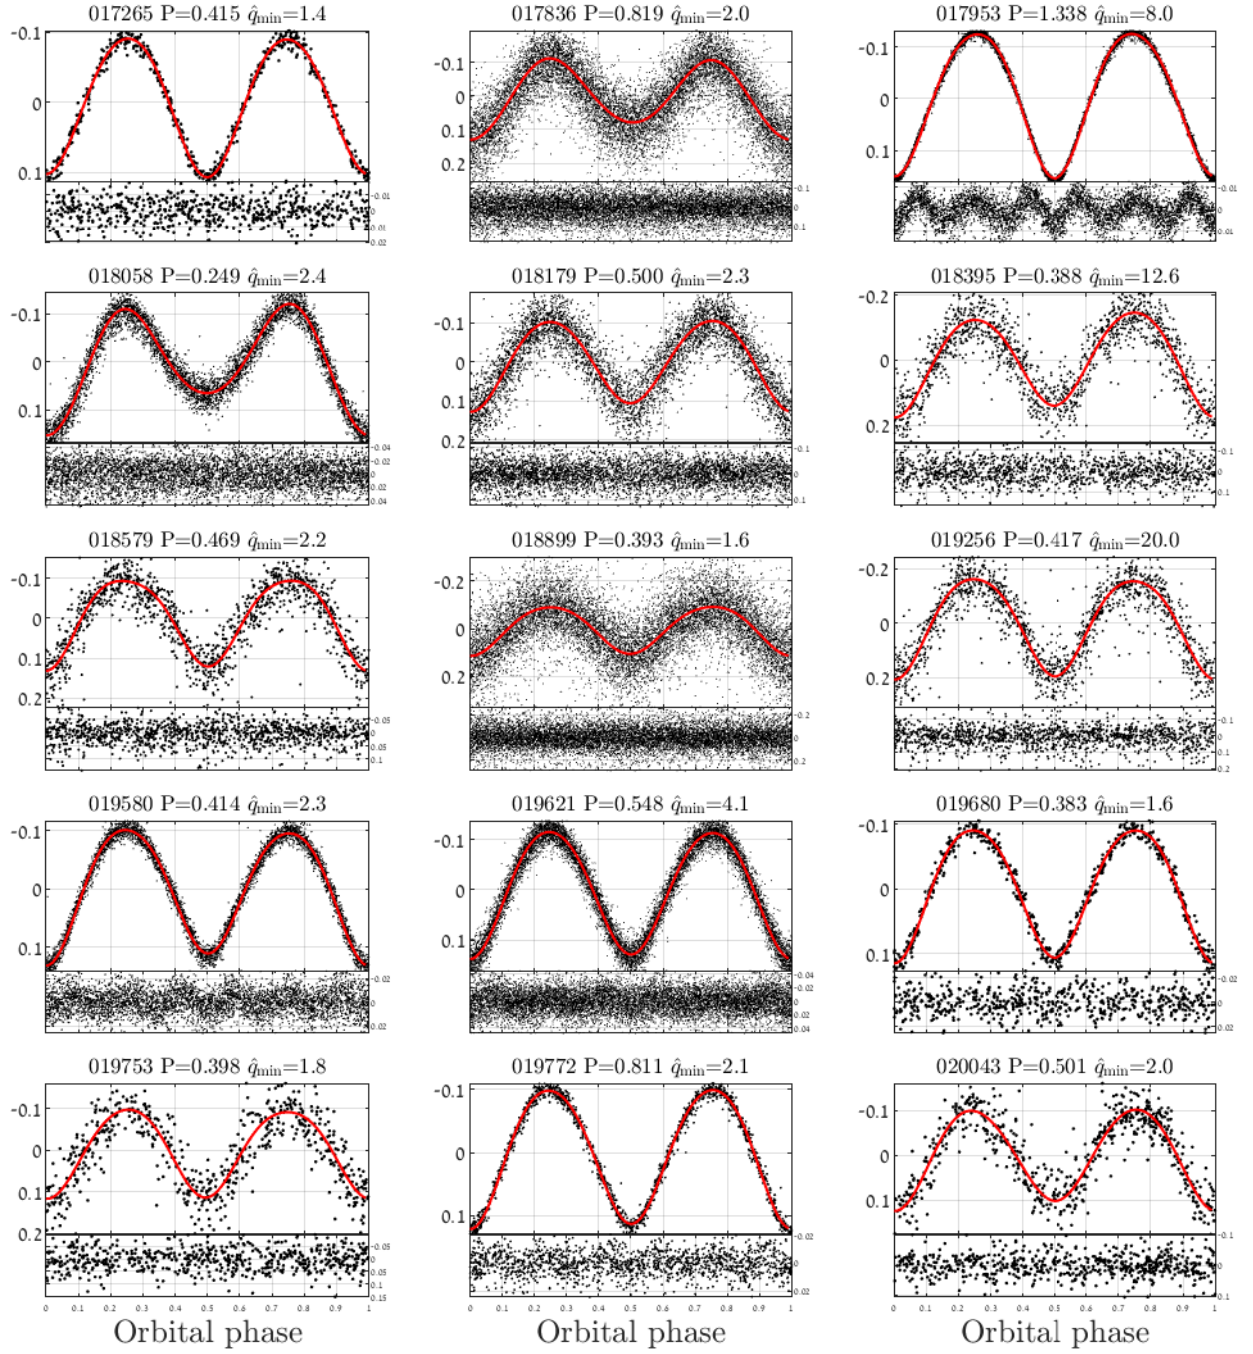

Figure S1. Continued

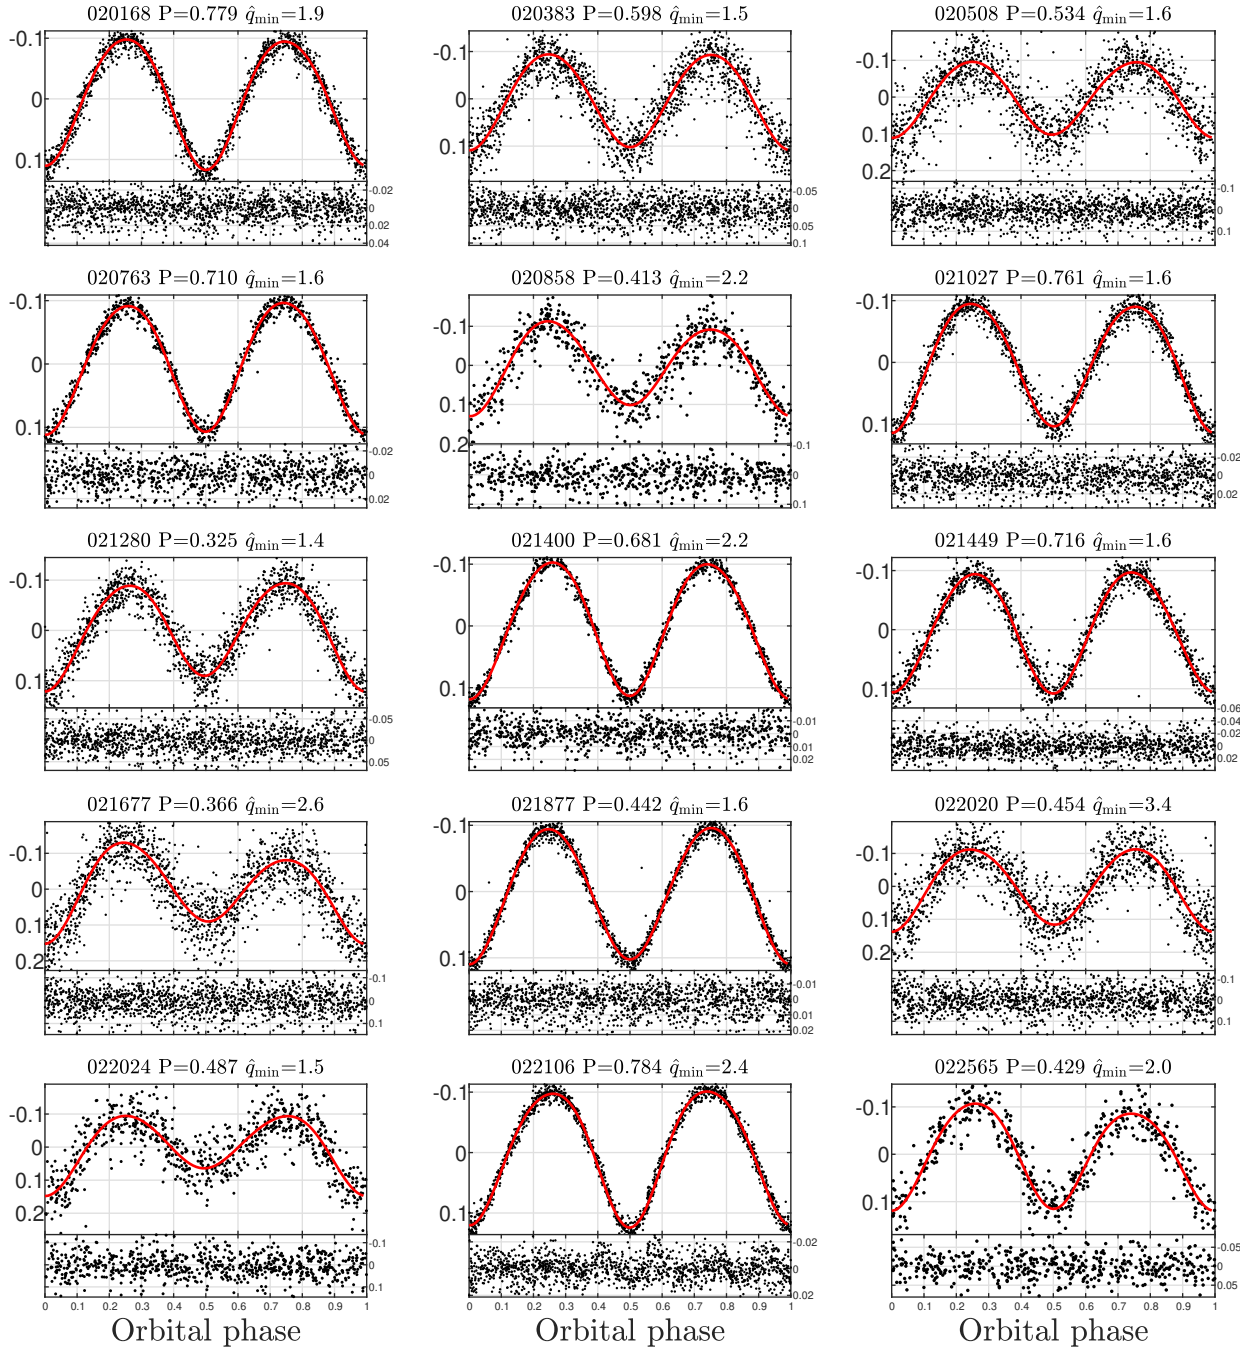

Figure S1. Continued



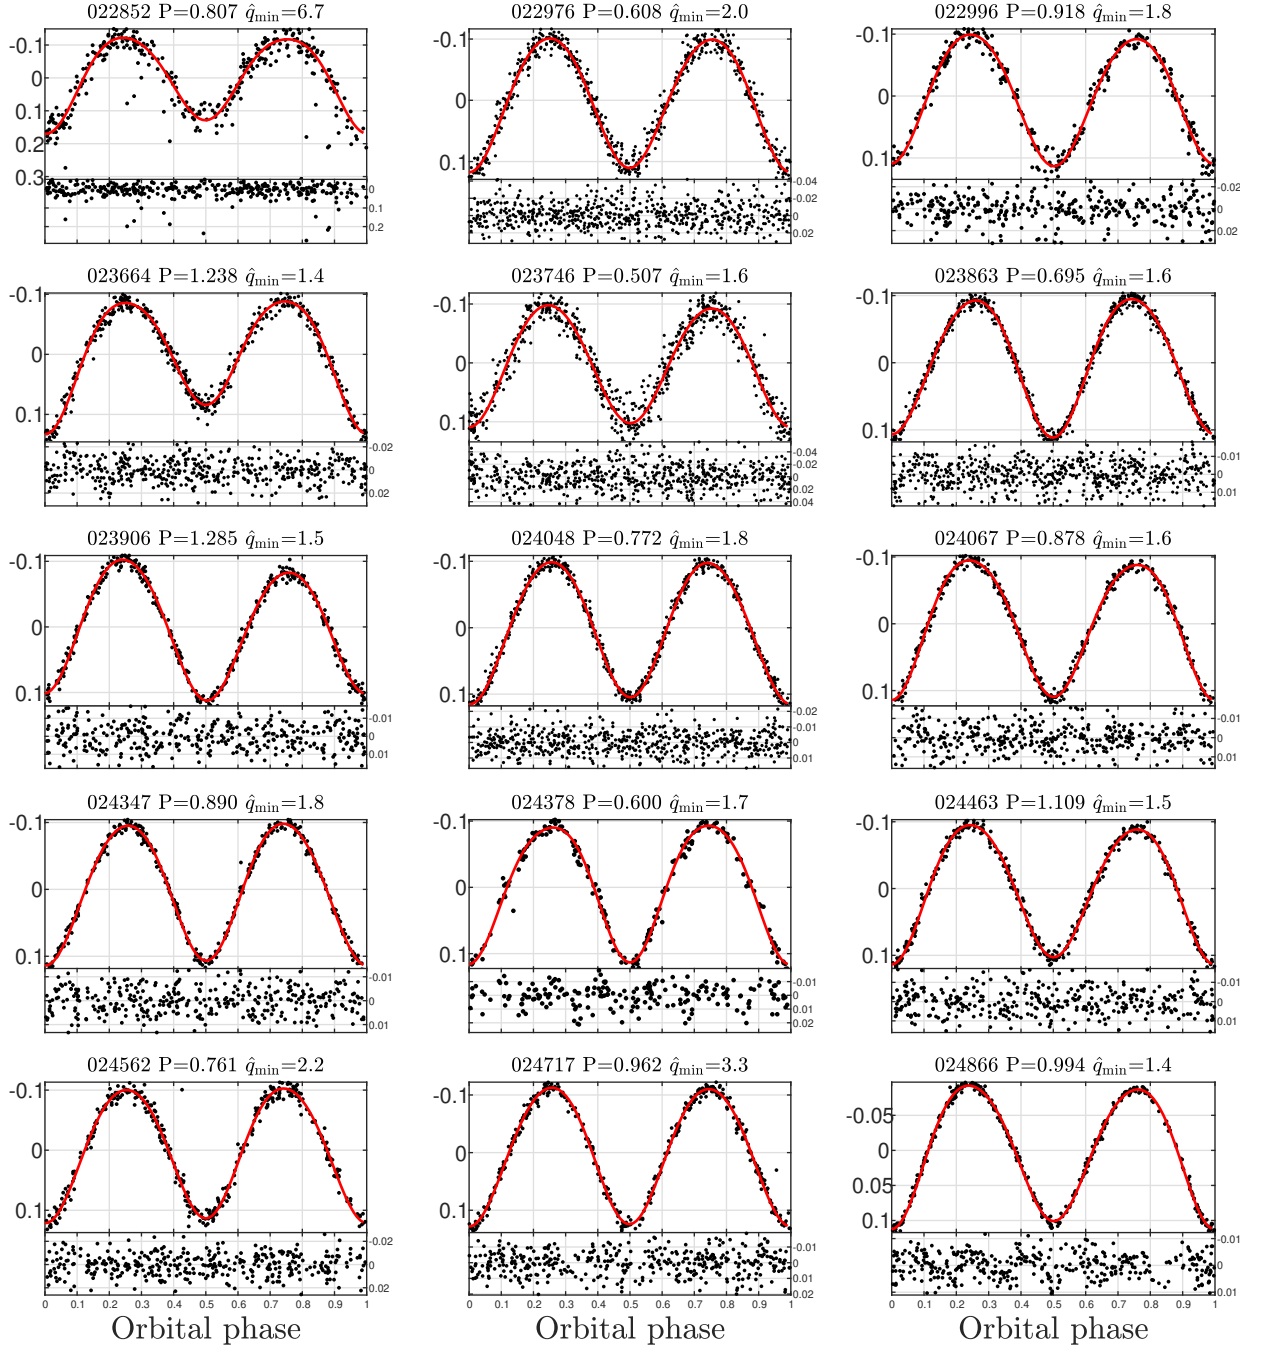

Figure S1. Continued

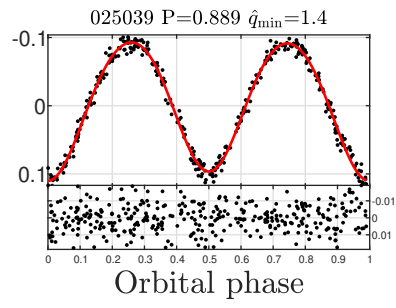

**Figure S1.** Continued

| ID     | P        | T <sub>0</sub> | I        | a <sub>1c</sub> | a <sub>2c</sub> | a <sub>3c</sub> | a <sub>4c</sub> | a <sub>1s</sub> | a <sub>2s</sub> | a <sub>3s</sub> | a <sub>4s</sub> | N    | N <sub>s</sub> | Δt   | χ <sub>red</sub> <sup>2</sup> | q <sub>min</sub> | q <sub>min</sub> <sup>-1σ</sup> |
|--------|----------|----------------|----------|-----------------|-----------------|-----------------|-----------------|-----------------|-----------------|-----------------|-----------------|------|----------------|------|-------------------------------|------------------|---------------------------------|
| 000001 | 0.182739 | 6171.72930     | 18.4002  | -0.0235         | 0.1187          | -0.0111         | 0.0005          | 0.0060          | 0.0000          | -0.0017         | -0.0034         | 579  | 6              | 2029 | 2.5                           | 3.3              | 2.2                             |
| 000008 | 0.213058 | 6393.89664     | 19.0265  | -0.0095         | 0.1019          | -0.0001         | -0.0090         | 0.0016          | 0.0000          | 0.0015          | -0.0021         | 4995 | 6              | 2072 | 2.8                           | 1.7              | 1.2                             |
| 000010 | 0.217000 | 6392.91249     | 18.18486 | -0.02337        | 0.10130         | -0.01197        | 0.00212         | -0.01026        | 0.00000         | -0.00182        | -0.00203        | 4972 | 6              | 2072 | 3.7                           | 1.6              | 1.2                             |
| 000014 | 0.198242 | 6117.20526     | 17.8945  | -0.0128         | 0.0994          | -0.0148         | 0.0036          | -0.0056         | 0.0000          | -0.0015         | -0.0022         | 646  | 6              | 2069 | 3.1                           | 1.5              | 1.1                             |
| 000052 | 0.387288 | 5790.6487      | 18.2595  | -0.0095         | 0.1246          | -0.0110         | -0.0066         | 0.0019          | 0.0000          | -0.0066         | -0.0084         | 271  | 4              | 1311 | 2.4                           | 4.3              | 2.7                             |
| 000090 | 0.545850 | 2729.8142      | 17.7955  | -0.0094         | 0.0985          | -0.0035         | -0.0021         | 0.0014          | 0.0000          | 0.0073          | -0.0038         | 100  | 2              | 593  | 1.2                           | 1.5              | 1.0                             |
| 000190 | 0.424034 | 5788.36752     | 14.72946 | -0.0071         | 0.1571          | -0.0046         | -0.0228         | 0.0004          | 0.0000          | -0.0007         | 0.0001          | 270  | 4              | 1311 | 22                            | 20               | 11                              |
| 000079 | 0.522313 | 6169.7456      | 18.1462  | -0.0022         | 0.1120          | -0.0049         | -0.0088         | -0.0003         | 0.0000          | 0.0023          | -0.0011         | 581  | 6              | 2029 | 3.4                           | 2.5              | 1.7                             |
| 000717 | 1.249635 | 2555.5971      | 17.4605  | -0.0085         | 0.1009          | 0.0078          | -0.0038         | -0.0032         | 0.0000          | 0.0000          | -0.0021         | 98   | 2              | 598  | 1.9                           | 1.6              | 1.1                             |
| 001458 | 0.577088 | 6178.3318      | 18.8606  | -0.0135         | 0.1073          | -0.0033         | -0.0087         | -0.0026         | 0.0000          | -0.0009         | -0.0013         | 576  | 6              | 2047 | 2.7                           | 2.1              | 1.4                             |
| 001673 | 0.908019 | 6220.92755     | 18.50546 | -0.00575        | 0.10429         | 0.00268         | -0.00660        | -0.00047        | 0.00000         | 0.00092         | -0.00036        | 4602 | 6              | 2055 | 2.5                           | 1.8              | 1.3                             |
| 001825 | 0.734745 | 6457.9357      | 16.2996  | -0.0115         | 0.1114          | -0.0077         | -0.0109         | 0.0023          | 0.0000          | 0.0007          | 0.0016          | 286  | 5              | 1671 | 35                            | 2.4              | 1.7                             |
| 001861 | 1.149962 | 6377.9891      | 19.1131  | -0.0144         | 0.1278          | -0.0053         | -0.0115         | 0.0014          | 0.0000          | -0.0003         | 0.0012          | 4800 | 6              | 2055 | 2.6                           | 4.9              | 3.1                             |
| 001967 | 0.428522 | 6427.0104      | 19.7377  | -0.0030         | 0.1240          | 0.0042          | -0.0112         | -0.0006         | 0.0000          | -0.0019         | -0.0034         | 4286 | 6              | 2052 | 3.0                           | 4.2              | 2.6                             |
| 002327 | 0.842062 | 6378.93513     | 18.81913 | -0.0095         | 0.1008          | -0.0057         | -0.0083         | 0.0020          | 0.0000          | 0.0011          | -0.0021         | 4809 | 6              | 2055 | 3.1                           | 1.6              | 1.1                             |

**Table S1.** Fitted parameters of our 136 candidates: OGLE ID (last six digits), OGLE orbital period [days], reference time [JD-2450000], reference-time error, fitted I magnitude, fitted I magnitude error, cosine and sine Fourier coefficients, each followed by its error [mag], total number of analyzed points, total number of analyzed seasons, light-curve time range [days], reduced  $\chi^2$  of the four-harmonic model, mMMR and lower-percentile mMMR. The full table is available at the CDS.

| ID     | $P$      | $T_0$<br>$T_{0, \text{err}}$ | $I$<br>$I_{\text{err}}$ | $a_{1c}$<br>$a_{1c, \text{err}}$ | $a_{2c}$<br>$a_{2c, \text{err}}$ | $a_{3c}$<br>$a_{3c, \text{err}}$ | $a_{4c}$<br>$a_{4c, \text{err}}$ | $a_{1s}$<br>$a_{1s, \text{err}}$ | $a_{2s}$<br>$a_{2s, \text{err}}$ | $a_{3s}$<br>$a_{3s, \text{err}}$ | $a_{4s}$<br>$a_{4s, \text{err}}$ | $N$  | $N_s$ | $\Delta t$ | $\chi^2_{\text{red}}$ | $\hat{q}_{\text{min}}$ | $\hat{q}_{\text{min}}^{-1\sigma}$ |
|--------|----------|------------------------------|-------------------------|----------------------------------|----------------------------------|----------------------------------|----------------------------------|----------------------------------|----------------------------------|----------------------------------|----------------------------------|------|-------|------------|-----------------------|------------------------|-----------------------------------|
| 002458 | 1.103268 | 6374.7507<br>0.0011          | 18.91578<br>0.00095     | -0.0132<br>0.0014                | 0.1128<br>0.0014                 | -0.0077<br>0.0013                | -0.0022<br>0.0013                | -0.0007<br>0.0013                | 0.0000<br>0.0013                 | 0.0007<br>0.0014                 | -0.0002<br>0.0014                | 4750 | 6     | 2055       | 3.1                   | 2.6                    | 1.8                               |
| 002483 | 0.532113 | 6379.1481<br>0.0012          | 19.4086<br>0.0016       | -0.0284<br>0.0024                | 0.1020<br>0.0023                 | -0.0046<br>0.0022                | -0.0046<br>0.0023                | 0.0043<br>0.0021                 | 0.0000<br>0.0022                 | 0.0029<br>0.0022                 | 0.0010<br>0.0022                 | 4810 | 6     | 2055       | 2.6                   | 1.7                    | 1.2                               |
| 002860 | 0.631836 | 6378.2157<br>0.0013          | 19.4982<br>0.0016       | -0.0088<br>0.0023                | 0.0986<br>0.0022                 | -0.0055<br>0.0022                | -0.0004<br>0.0022                | -0.0039<br>0.0021                | 0.0000<br>0.0022                 | 0.0006<br>0.0022                 | -0.0033<br>0.0022                | 4801 | 6     | 2055       | 3.0                   | 1.5                    | 1.0                               |
| 003067 | 0.463240 | 6103.89842<br>0.0023         | 16.75731<br>0.0052      | -0.00670<br>0.00078              | 0.13004<br>0.00077               | -0.00421<br>0.00077              | -0.00794<br>0.00075              | -0.00057<br>0.00071              | 0.00000<br>0.00073               | -0.00073<br>0.00072              | -0.00049<br>0.00074              | 613  | 6     | 2048       | 3.4                   | 5.5                    | 3.4                               |
| 003074 | 0.962841 | 6071.16957<br>0.0058         | 16.35892<br>0.0044      | -0.00595<br>0.00065              | 0.11153<br>0.00063               | 0.00372<br>0.00064               | -0.01041<br>0.00064              | -0.00182<br>0.00060              | 0.00000<br>0.00062               | -0.00088<br>0.00061              | 0.00098<br>0.00061               | 546  | 6     | 2030       | 2.0                   | 2.5                    | 1.7                               |
| 004427 | 0.705079 | 6349.34936<br>0.0039         | 13.70541<br>0.0036      | 0.00657<br>0.00053               | 0.10409<br>0.00052               | -0.00331<br>0.00050              | -0.00983<br>0.00053              | 0.00849<br>0.00049               | 0.00000<br>0.00050               | -0.00025<br>0.00052              | 0.00050<br>0.00050               | 349  | 6     | 2037       | 2.6                   | 1.8                    | 1.3                               |
| 004476 | 0.775191 | 6116.86629<br>0.0033         | 15.45266<br>0.0031      | -0.00750<br>0.00046              | 0.10550<br>0.00045               | 0.00365<br>0.00044               | -0.00913<br>0.00044              | -0.00038<br>0.00043              | 0.00000<br>0.00044               | -0.00101<br>0.00045              | 0.00003<br>0.00045               | 641  | 6     | 2053       | 2.9                   | 1.9                    | 1.4                               |
| 004738 | 0.901710 | 2842.13954<br>0.0049         | 13.32283<br>0.0045      | 0.00357<br>0.00064               | 0.11052<br>0.00065               | -0.00419<br>0.00064              | -0.01082<br>0.00064              | 0.00495<br>0.00064               | 0.00000<br>0.00063               | 0.00058<br>0.00063               | 0.00009<br>0.00062               | 228  | 2     | 587        | 1.8                   | 2.4                    | 1.6                               |
| 004755 | 0.362357 | 6786.48706<br>0.0069         | 16.3770<br>0.0016       | -0.0025<br>0.0022                | 0.1127<br>0.0021                 | 0.0025<br>0.0022                 | -0.0118<br>0.0022                | -0.0005<br>0.0021                | 0.0000<br>0.0022                 | -0.0039<br>0.0022                | -0.0022<br>0.0021                | 100  | 1     | 229        | 4.0                   | 2.6                    | 1.7                               |
| 004787 | 0.461733 | 6363.9533<br>0.0020          | 18.9298<br>0.0033       | -0.0292<br>0.0051                | 0.1074<br>0.0048                 | -0.0084<br>0.0049                | 0.0007<br>0.0048                 | 0.0100<br>0.0045                 | 0.0000<br>0.0047                 | -0.0011<br>0.0046                | -0.0018<br>0.0047                | 353  | 6     | 2037       | 1.9                   | 2.1                    | 1.4                               |
| 005636 | 0.469911 | 6104.06811<br>0.0024         | 15.77619<br>0.0049      | -0.00312<br>0.00073              | 0.11120<br>0.00069               | -0.00475<br>0.00069              | -0.00721<br>0.00068              | 0.00047<br>0.00066               | 0.00000<br>0.00071               | 0.00052<br>0.00070               | -0.00055<br>0.00071              | 552  | 6     | 2046       | 3.4                   | 2.4                    | 1.7                               |
| 005844 | 0.641542 | 6348.94749<br>0.0028         | 14.60688<br>0.0036      | -0.00065<br>0.00052              | 0.10536<br>0.00050               | -0.00475<br>0.00053              | -0.01102<br>0.00052              | 0.00485<br>0.00052               | 0.00000<br>0.00053               | 0.00073<br>0.00051               | 0.00020<br>0.00051               | 349  | 6     | 2037       | 2.7                   | 1.9                    | 1.4                               |
| 005857 | 1.079872 | 6119.81295<br>0.0080         | 15.25195<br>0.0056      | -0.00322<br>0.00078              | 0.10517<br>0.00078               | 0.00292<br>0.00080               | -0.01118<br>0.00078              | 0.00017<br>0.00079               | 0.00000<br>0.00080               | -0.00009<br>0.00077              | -0.00141<br>0.00079              | 418  | 6     | 2046       | 7.1                   | 1.9                    | 1.3                               |
| 005990 | 0.553912 | 5834.81070<br>0.0056         | 16.25115<br>0.0077      | -0.0022<br>0.0011                | 0.1216<br>0.0011                 | -0.0063<br>0.0011                | -0.0124<br>0.0011                | 0.0018<br>0.0010                 | 0.0000<br>0.0011                 | -0.0002<br>0.0011                | -0.0025<br>0.0011                | 221  | 4     | 1312       | 1.9                   | 3.8                    | 2.4                               |
| 006007 | 1.354867 | 6436.28357<br>0.0056         | 15.62401<br>0.0037      | -0.00435<br>0.00053              | 0.10823<br>0.00052               | 0.00468<br>0.00051               | -0.00728<br>0.00052              | -0.00135<br>0.00051              | 0.00000<br>0.00052               | 0.00078<br>0.00053               | 0.00103<br>0.00052               | 434  | 6     | 2047       | 2.0                   | 2.1                    | 1.5                               |

Table S1. Continued

| ID     | $P$      | $T_0$      | $I$      | $a_{1c}$ | $a_{2c}$ | $a_{3c}$ | $a_{4c}$ | $a_{1s}$ | $a_{2s}$ | $a_{3s}$ | $a_{4s}$ | $N$   | $N_s$ | $\Delta t$ | $\chi^2_{\text{red}}$ | $\hat{q}_{\text{min}}$ | $\hat{q}_{\text{min}}^{1\sigma}$ |
|--------|----------|------------|----------|----------|----------|----------|----------|----------|----------|----------|----------|-------|-------|------------|-----------------------|------------------------|----------------------------------|
| 006183 | 0.353179 | 1300.5102  | 18.5894  | -0.0063  | 0.1255   | -0.0025  | -0.0051  | -0.0006  | 0.0000   | -0.0034  | -0.0017  | 310   | 4     | 1275       | 2.0                   | 4.5                    | 2.7                              |
|        |          | 0.0013     | 0.0034   | 0.0052   | 0.0050   | 0.0048   | 0.0048   | 0.0046   | 0.0048   | 0.0050   | 0.0049   |       |       |            |                       |                        |                                  |
| 006364 | 0.490059 | 6461.0098  | 18.6085  | 0.0015   | 0.1146   | 0.0005   | -0.0066  | 0.0047   | 0.0000   | 0.0038   | 0.0025   | 751   | 6     | 2057       | 8.8                   | 2.8                    | 1.8                              |
|        |          | 0.0016     | 0.0024   | 0.0036   | 0.0034   | 0.0035   | 0.0035   | 0.0033   | 0.0034   | 0.0034   | 0.0034   |       |       |            |                       |                        |                                  |
| 006500 | 0.523564 | 6376.0943  | 18.0802  | -0.0019  | 0.1311   | 0.0070   | -0.0016  | -0.0010  | 0.0000   | -0.0036  | 0.0011   | 1423  | 6     | 2054       | 6.2                   | 5.8                    | 3.5                              |
|        |          | 0.0011     | 0.0019   | 0.0028   | 0.0027   | 0.0026   | 0.0027   | 0.0025   | 0.0027   | 0.0027   | 0.0026   |       |       |            |                       |                        |                                  |
| 006667 | 0.900829 | 6175.2556  | 17.60383 | -0.0094  | 0.0997   | -0.0061  | -0.0067  | -0.0024  | 0.0000   | -0.0010  | -0.0011  | 828   | 6     | 2035       | 3.9                   | 1.5                    | 1.1                              |
|        |          | 0.0014     | 0.00099  | 0.0014   | 0.0014   | 0.0014   | 0.0014   | 0.0014   | 0.0014   | 0.0014   | 0.0014   |       |       |            |                       |                        |                                  |
| 006785 | 0.467160 | 6114.15577 | 15.78935 | -0.00240 | 0.10151  | -0.00462 | -0.00822 | 0.00079  | 0.00000  | -0.00020 | -0.00031 | 653   | 6     | 2073       | 3.2                   | 1.6                    | 1.2                              |
|        |          | 0.0019     | 0.00035  | 0.00049  | 0.00049  | 0.00049  | 0.00050  | 0.00049  | 0.00049  | 0.00049  | 0.00049  |       |       |            |                       |                        |                                  |
| 007595 | 1.008979 | 6364.73373 | 15.83833 | 0.00023  | 0.11502  | -0.00566 | -0.01141 | 0.00326  | 0.00000  | 0.00064  | -0.00046 | 1451  | 6     | 2072       | 3.2                   | 2.8                    | 1.9                              |
|        |          | 0.0029     | 0.00021  | 0.00031  | 0.00030  | 0.00030  | 0.00030  | 0.00030  | 0.00030  | 0.00030  | 0.00030  |       |       |            |                       |                        |                                  |
| 007606 | 0.892979 | 6348.7314  | 18.8454  | -0.0153  | 0.1072   | -0.0066  | -0.0065  | 0.0033   | 0.0000   | 0.0015   | 0.0013   | 1473  | 6     | 2071       | 2.2                   | 2.1                    | 1.4                              |
|        |          | 0.0022     | 0.0016   | 0.0025   | 0.0024   | 0.0023   | 0.0023   | 0.0022   | 0.0023   | 0.0024   | 0.0024   |       |       |            |                       |                        |                                  |
| 007774 | 0.876233 | 6438.4371  | 19.33892 | -0.0248  | 0.1053   | -0.0039  | -0.0120  | 0.0064   | 0.0000   | 0.0010   | -0.0029  | 12013 | 6     | 2012       | 2.8                   | 1.9                    | 1.3                              |
|        |          | 0.0012     | 0.00088  | 0.0013   | 0.0013   | 0.0013   | 0.0013   | 0.0012   | 0.0012   | 0.0012   | 0.0012   |       |       |            |                       |                        |                                  |
| 007878 | 0.656309 | 6363.3508  | 18.5608  | -0.0171  | 0.1291   | -0.0113  | -0.0098  | -0.0014  | 0.0000   | -0.0010  | -0.0024  | 1451  | 6     | 2072       | 5.2                   | 5.3                    | 3.2                              |
|        |          | 0.0013     | 0.0017   | 0.0025   | 0.0024   | 0.0023   | 0.0023   | 0.0022   | 0.0023   | 0.0024   | 0.0024   |       |       |            |                       |                        |                                  |
| 008074 | 1.001498 | 6374.83691 | 14.36264 | -0.00725 | 0.10681  | 0.00354  | -0.00515 | 0.00400  | 0.00000  | 0.00000  | 0.00102  | 352   | 6     | 2047       | 1.8                   | 2.0                    | 1.4                              |
|        |          | 0.0041     | 0.00032  | 0.00041  | 0.00046  | 0.00044  | 0.00045  | 0.00056  | 0.00045  | 0.00045  | 0.00044  |       |       |            |                       |                        |                                  |
| 008274 | 0.487881 | 6211.84608 | 16.01828 | -0.00013 | 0.10528  | -0.00269 | -0.01141 | 0.00093  | 0.00000  | 0.00043  | -0.00029 | 1387  | 6     | 2071       | 3.7                   | 1.9                    | 1.3                              |
|        |          | 0.0021     | 0.00028  | 0.00041  | 0.00040  | 0.00040  | 0.00039  | 0.00039  | 0.00039  | 0.00040  | 0.00040  |       |       |            |                       |                        |                                  |
| 008323 | 0.792437 | 6410.05215 | 18.60458 | -0.0095  | 0.1099   | -0.0047  | -0.0175  | -0.0024  | 0.0000   | 0.0010   | -0.0009  | 12740 | 6     | 2073       | 6.0                   | 2.3                    | 1.6                              |
|        |          | 0.00085    | 0.00079  | 0.0012   | 0.0011   | 0.0011   | 0.0011   | 0.0011   | 0.0011   | 0.0011   | 0.0011   |       |       |            |                       |                        |                                  |
| 008919 | 0.551739 | 5828.01850 | 15.71142 | -0.00232 | 0.10277  | 0.00318  | -0.00736 | -0.00024 | 0.00000  | 0.00034  | -0.00140 | 218   | 4     | 1321       | 2.3                   | 1.7                    | 1.2                              |
|        |          | 0.00055    | 0.00066  | 0.00094  | 0.00094  | 0.00090  | 0.00092  | 0.00091  | 0.00091  | 0.00095  | 0.00092  |       |       |            |                       |                        |                                  |
| 008968 | 0.967032 | 6381.4369  | 19.2308  | -0.0166  | 0.1031   | -0.0079  | -0.0035  | 0.0023   | 0.0000   | -0.0016  | 0.0006   | 4891  | 6     | 2072       | 2.8                   | 1.7                    | 1.2                              |
|        |          | 0.0019     | 0.0013   | 0.0019   | 0.0018   | 0.0018   | 0.0018   | 0.0017   | 0.0018   | 0.0018   | 0.0018   |       |       |            |                       |                        |                                  |
| 009330 | 0.616125 | 6401.01153 | 14.51353 | -0.00773 | 0.10350  | 0.00282  | -0.00932 | -0.00131 | 0.00000  | -0.00054 | -0.00003 | 525   | 6     | 2057       | 2.6                   | 1.8                    | 1.3                              |
|        |          | 0.0020     | 0.00029  | 0.00041  | 0.00041  | 0.00041  | 0.00042  | 0.00041  | 0.00041  | 0.00041  | 0.00040  |       |       |            |                       |                        |                                  |

Table S1. Continued

| ID     | $P$      | $T_0$<br>$T_{0,err}$   | $I$<br>$I_{err}$    | $a_{1c}$<br>$a_{1c,err}$ | $a_{2c}$<br>$a_{2c,err}$ | $a_{3c}$<br>$a_{3c,err}$ | $a_{4c}$<br>$a_{4c,err}$ | $a_{1s}$<br>$a_{1s,err}$ | $a_{2s}$<br>$a_{2s,err}$ | $a_{3s}$<br>$a_{3s,err}$ | $a_{4s}$<br>$a_{4s,err}$ | $N$   | $N_s$ | $\Delta t$ | $\chi^2_{red}$ | $\hat{q}_{min}$ | $\hat{q}_{min}^{-1\sigma}$ |
|--------|----------|------------------------|---------------------|--------------------------|--------------------------|--------------------------|--------------------------|--------------------------|--------------------------|--------------------------|--------------------------|-------|-------|------------|----------------|-----------------|----------------------------|
| 009419 | 0.941939 | 6398.3003<br>0.0012    | 18.8639<br>0.0010   | -0.0141<br>0.0015        | 0.1092<br>0.0014         | -0.0055<br>0.0014        | -0.0163<br>0.0014        | 0.0005<br>0.0014         | 0.0000<br>0.0014         | 0.0017<br>0.0014         | 0.0033<br>0.0014         | 4882  | 6     | 2070       | 3.0            | 2.2             | 1.5                        |
| 009485 | 0.461473 | 6378.837217<br>0.00093 | 15.11593<br>0.00016 | 0.00282<br>0.00023       | 0.10361<br>0.00023       | 0.00279<br>0.00023       | -0.00859<br>0.00023      | 0.00329<br>0.00023       | 0.00000<br>0.00023       | -0.00009<br>0.00023      | -0.00029<br>0.00023      | 4897  | 6     | 2071       | 7.9            | 1.8             | 1.3                        |
| 009548 | 0.503039 | 6432.95788<br>0.00063  | 18.8676<br>0.0011   | -0.0136<br>0.0016        | 0.1046<br>0.0015         | -0.0060<br>0.0015        | -0.0073<br>0.0015        | 0.0001<br>0.0015         | 0.0000<br>0.0015         | 0.0023<br>0.0015         | 0.0006<br>0.0015         | 3696  | 6     | 2066       | 3.0            | 1.9             | 1.3                        |
| 009698 | 0.455461 | 6407.19480<br>0.00051  | 19.07265<br>0.00086 | -0.0072<br>0.0013        | 0.1242<br>0.0012         | -0.0075<br>0.0012        | -0.0126<br>0.0012        | 0.0013<br>0.0012         | 0.0000<br>0.0012         | 0.0006<br>0.0012         | 0.0008<br>0.0012         | 12660 | 6     | 2073       | 3.8            | 4.2             | 2.7                        |
| 009989 | 0.585696 | 6361.9251<br>0.0013    | 18.5858<br>0.0014   | -0.0159<br>0.0021        | 0.1003<br>0.0021         | -0.0064<br>0.0021        | -0.0061<br>0.0020        | -0.0024<br>0.0019        | 0.0000<br>0.0020         | 0.0001<br>0.0020         | -0.0032<br>0.0020        | 1443  | 6     | 2072       | 3.0            | 1.6             | 1.1                        |
| 010170 | 0.475805 | 6377.03738<br>0.00027  | 12.46143<br>0.00047 | -0.00269<br>0.00067      | 0.11788<br>0.00065       | -0.00329<br>0.00068      | -0.01426<br>0.00069      | 0.00035<br>0.00066       | 0.00000<br>0.00069       | -0.00071<br>0.00066      | 0.00088<br>0.00065       | 353   | 6     | 2047       | 5.8            | 3.2             | 2.1                        |
| 010848 | 0.231484 | 6308.95935<br>0.00023  | 18.27743<br>0.00076 | -0.0295<br>0.0011        | 0.0997<br>0.0011         | -0.0118<br>0.0011        | 0.0042<br>0.0011         | -0.0103<br>0.0010        | 0.0000<br>0.0011         | 0.0007<br>0.0011         | -0.0003<br>0.0011        | 4901  | 6     | 2074       | 3.9            | 1.5             | 1.1                        |
| 010985 | 0.321676 | 6407.390134<br>0.00090 | 16.59071<br>0.00035 | -0.00511<br>0.00052      | 0.19427<br>0.00050       | 0.00343<br>0.00049       | -0.01892<br>0.00050      | 0.00852<br>0.00047       | 0.00000<br>0.00049       | 0.00037<br>0.00049       | -0.00028<br>0.00049      | 4616  | 6     | 2071       | 11             | 20              | 20                         |
| 011277 | 0.741104 | 5823.5897<br>0.0013    | 19.2782<br>0.0013   | -0.0011<br>0.0019        | 0.1000<br>0.0018         | -0.0002<br>0.0018        | -0.0039<br>0.0018        | 0.0032<br>0.0017         | 0.0000<br>0.0018         | 0.0004<br>0.0018         | 0.0020<br>0.0018         | 7103  | 6     | 2073       | 5.1            | 1.5             | 1.1                        |
| 011652 | 0.523215 | 6373.07689<br>0.00057  | 18.48659<br>0.00074 | 0.0006<br>0.0011         | 0.0980<br>0.0011         | -0.0016<br>0.0011        | -0.0064<br>0.0010        | 0.0016<br>0.0010         | 0.0000<br>0.0010         | -0.0014<br>0.0011        | 0.0004<br>0.0011         | 4972  | 6     | 2074       | 2.2            | 1.4             | 1.0                        |
| 011720 | 0.757849 | 5821.02699<br>0.00100  | 19.08281<br>0.00098 | -0.0151<br>0.0015        | 0.1118<br>0.0014         | -0.0073<br>0.0014        | -0.0061<br>0.0014        | 0.0021<br>0.0013         | 0.0000<br>0.0014         | 0.0023<br>0.0014         | -0.0010<br>0.0014        | 7080  | 6     | 2073       | 3.5            | 2.5             | 1.7                        |
| 011740 | 0.508504 | 6416.26330<br>0.00031  | 18.42094<br>0.00044 | -0.00177<br>0.00065      | 0.10236<br>0.00063       | -0.00209<br>0.00062      | -0.00813<br>0.00062      | -0.00070<br>0.00060      | 0.00000<br>0.00062       | 0.00120<br>0.00062       | -0.00105<br>0.00062      | 12728 | 6     | 2073       | 2.3            | 1.7             | 1.2                        |
| 012265 | 1.050083 | 5824.36932<br>0.00098  | 17.91530<br>0.00064 | -0.00677<br>0.00094      | 0.10706<br>0.00091       | 0.00430<br>0.00090       | -0.00831<br>0.00090      | 0.00224<br>0.00087       | 0.00000<br>0.00090       | 0.00071<br>0.00090       | 0.00040<br>0.00090       | 7094  | 6     | 2073       | 6.4            | 2.0             | 1.4                        |
| 012306 | 0.895213 | 6100.26505<br>0.00046  | 13.06907<br>0.00037 | -0.00089<br>0.00053      | 0.11219<br>0.00053       | -0.00448<br>0.00054      | -0.00728<br>0.00052      | 0.00335<br>0.00052       | 0.00000<br>0.00053       | 0.00016<br>0.00052       | -0.00091<br>0.00053      | 649   | 6     | 2069       | 6.0            | 2.5             | 1.7                        |
| 012446 | 0.392024 | 5820.68629<br>0.00018  | 17.61300<br>0.00041 | -0.00492<br>0.00061      | 0.11875<br>0.00058       | -0.00516<br>0.00058      | -0.01308<br>0.00057      | -0.00033<br>0.00055      | 0.00000<br>0.00058       | 0.00037<br>0.00058       | -0.00043<br>0.00058      | 7103  | 6     | 2073       | 5.2            | 3.3             | 2.2                        |

Table S1. Continued



| ID     | $P$      | $T_0$<br>$T_{0,err}$    | $I$<br>$I_{err}$    | $a_{1c}$<br>$a_{1c,err}$ | $a_{2c}$<br>$a_{2c,err}$ | $a_{3c}$<br>$a_{3c,err}$ | $a_{4c}$<br>$a_{4c,err}$ | $a_{1s}$<br>$a_{1s,err}$ | $a_{2s}$<br>$a_{2s,err}$ | $a_{3s}$<br>$a_{3s,err}$ | $a_{4s}$<br>$a_{4s,err}$ | $N$   | $N_s$ | $\Delta t$ | $\chi^2_{red}$ | $\hat{q}_{min}$ | $\hat{q}_{min}^{-1\sigma}$ |
|--------|----------|-------------------------|---------------------|--------------------------|--------------------------|--------------------------|--------------------------|--------------------------|--------------------------|--------------------------|--------------------------|-------|-------|------------|----------------|-----------------|----------------------------|
| 012599 | 0.413567 | 5965.18820<br>0.00052   | 19.0923<br>0.0011   | -0.0012<br>0.0017        | 0.1052<br>0.0016         | 0.0007<br>0.0016         | -0.0127<br>0.0016        | 0.0047<br>0.0016         | 0.0000<br>0.0016         | 0.0003<br>0.0016         | -0.0006<br>0.0016        | 6249  | 6     | 2073       | 3.4            | 1.9             | 1.3                        |
| 013181 | 1.350592 | 6354.6486<br>0.0032     | 18.7660<br>0.0028   | -0.0159<br>0.0043        | 0.1414<br>0.0041         | -0.0131<br>0.0040        | -0.0140<br>0.0040        | -0.0064<br>0.0037        | 0.0000<br>0.0040         | -0.0069<br>0.0040        | 0.0087<br>0.0040         | 391   | 6     | 2044       | 2.2            | 9.7             | 5.2                        |
| 013249 | 0.472360 | 6416.74849<br>0.00014   | 17.62289<br>0.00026 | -0.00167<br>0.00038      | 0.10210<br>0.00036       | -0.00296<br>0.00036      | -0.00821<br>0.00036      | 0.00232<br>0.00035       | 0.00000<br>0.00036       | 0.00007<br>0.00036       | -0.00066<br>0.00036      | 12747 | 6     | 2073       | 2.6            | 1.7             | 1.2                        |
| 013256 | 0.518054 | 6419.06620<br>0.00038   | 18.63905<br>0.00053 | -0.00323<br>0.00079      | 0.10691<br>0.00076       | -0.00508<br>0.00076      | -0.00905<br>0.00075      | 0.00120<br>0.00072       | 0.00000<br>0.00075       | -0.00111<br>0.00075      | -0.00097<br>0.00075      | 12473 | 6     | 2073       | 2.6            | 2.0             | 1.4                        |
| 013257 | 0.999907 | 6416.9341<br>0.0054     | 16.8015<br>0.0026   | -0.0087<br>0.0016        | 0.1173<br>0.0078         | -0.0019<br>0.0017        | 0.0058<br>0.0012         | 0.078<br>0.011           | 0.0000<br>0.0021         | -0.0300<br>0.0039        | 0.00114<br>0.00073       | 12747 | 6     | 2073       | 3.1            | 3.1             | 1.9                        |
| 013402 | 0.384512 | 6416.07908<br>0.00030   | 18.68802<br>0.00075 | 0.0015<br>0.0011         | 0.1091<br>0.0011         | 0.0041<br>0.0011         | -0.0067<br>0.0011        | 0.0014<br>0.0010         | 0.0000<br>0.0011         | 0.0000<br>0.0011         | -0.0006<br>0.0011        | 12713 | 6     | 2073       | 4.6            | 2.2             | 1.5                        |
| 013501 | 0.428857 | 6409.99003<br>0.00021   | 18.06420<br>0.00034 | -0.00398<br>0.00051      | 0.11073<br>0.00049       | -0.00443<br>0.00048      | -0.01215<br>0.00048      | 0.00004<br>0.00046       | 0.00000<br>0.00048       | 0.00112<br>0.00049       | -0.00109<br>0.00049      | 12691 | 6     | 2073       | 2.8            | 2.4             | 1.6                        |
| 013800 | 0.415960 | 6367.97902<br>0.00079   | 18.9687<br>0.0012   | -0.0031<br>0.0018        | 0.1011<br>0.0017         | -0.0017<br>0.0017        | -0.0084<br>0.0017        | -0.0019<br>0.0016        | 0.0000<br>0.0017         | 0.0010<br>0.0017         | 0.0002<br>0.0017         | 4945  | 6     | 2074       | 3.0            | 1.6             | 1.1                        |
| 014265 | 0.692935 | 5392.5768<br>0.0017     | 17.5462<br>0.0023   | -0.0118<br>0.0034        | 0.1052<br>0.0033         | -0.0034<br>0.0032        | -0.0027<br>0.0032        | -0.0051<br>0.0031        | 0.0000<br>0.0032         | -0.0034<br>0.0032        | 0.0012<br>0.0032         | 1431  | 3     | 1330       | 44             | 1.9             | 1.3                        |
| 014329 | 0.508880 | 6415.98060<br>0.00036   | 18.17851<br>0.00046 | -0.00323<br>0.00068      | 0.09996<br>0.00065       | 0.00099<br>0.00065       | -0.00805<br>0.00065      | 0.00403<br>0.00062       | 0.00000<br>0.00065       | -0.00023<br>0.00065      | 0.00018<br>0.00065       | 12701 | 6     | 2073       | 3.4            | 1.5             | 1.1                        |
| 014523 | 0.450318 | 5823.889494<br>0.000071 | 15.20878<br>0.00011 | -0.00118<br>0.00015      | 0.10452<br>0.00015       | 0.00208<br>0.00015       | -0.00529<br>0.00015      | 0.00128<br>0.00015       | 0.00000<br>0.00015       | -0.00009<br>0.00015      | -0.00012<br>0.00015      | 7127  | 6     | 2073       | 5.0            | 1.8             | 1.3                        |
| 014566 | 0.806090 | 6125.79789<br>0.00045   | 16.44556<br>0.00037 | -0.00949<br>0.00053      | 0.10853<br>0.00053       | 0.00270<br>0.00053       | -0.00742<br>0.00053      | 0.00386<br>0.00051       | 0.00000<br>0.00051       | -0.00009<br>0.00051      | -0.00003<br>0.00051      | 1300  | 6     | 2072       | 3.7            | 1.8             | 1.3                        |
| 014686 | 0.968662 | 6062.61487<br>0.00041   | 16.09618<br>0.00036 | -0.00116<br>0.00051      | 0.10477<br>0.00050       | 0.00357<br>0.00050       | -0.01063<br>0.00051      | -0.00080<br>0.00050      | 0.00000<br>0.00050       | 0.00044<br>0.00050       | -0.00001<br>0.00050      | 590   | 6     | 2040       | 1.5            | 1.9             | 1.3                        |
| 015078 | 0.481804 | 6417.04862<br>0.00048   | 18.86477<br>0.00076 | 0.0010<br>0.0011         | 0.0978<br>0.0011         | 0.0041<br>0.0011         | -0.0061<br>0.0011        | 0.0022<br>0.0010         | 0.0000<br>0.0011         | -0.0015<br>0.0011        | -0.0013<br>0.0011        | 12747 | 6     | 2073       | 2.5            | 1.4             | 1.0                        |
| 015204 | 0.555361 | 6416.18076<br>0.00055   | 18.89608<br>0.00077 | -0.0087<br>0.0012        | 0.1085<br>0.0011         | -0.0052<br>0.0011        | -0.0084<br>0.0011        | 0.0003<br>0.0010         | 0.0000<br>0.0011         | -0.0001<br>0.0011        | -0.0014<br>0.0011        | 12708 | 6     | 2073       | 3.1            | 2.2             | 1.5                        |

Table S1. Continued

| ID     | P        | $T_0$<br>$T_{0, \text{err}}$ | I<br>$I_{\text{err}}$ | $a_{1c}$<br>$a_{1c, \text{err}}$ | $a_{2c}$<br>$a_{2c, \text{err}}$ | $a_{3c}$<br>$a_{3c, \text{err}}$ | $a_{4c}$<br>$a_{4c, \text{err}}$ | $a_{1s}$<br>$a_{1s, \text{err}}$ | $a_{2s}$<br>$a_{2s, \text{err}}$ | $a_{3s}$<br>$a_{3s, \text{err}}$ | $a_{4s}$<br>$a_{4s, \text{err}}$ | N     | $N_s$ | $\Delta t$ | $\chi^2_{\text{red}}$ | $\hat{q}_{\text{min}}$ | $\hat{q}_{\text{min}}^{-1\sigma}$ |
|--------|----------|------------------------------|-----------------------|----------------------------------|----------------------------------|----------------------------------|----------------------------------|----------------------------------|----------------------------------|----------------------------------|----------------------------------|-------|-------|------------|-----------------------|------------------------|-----------------------------------|
| 015369 | 0.272296 | 6057.95348<br>0.00024        | 18.43903<br>0.00071   | -0.0162<br>0.0011                | 0.1025<br>0.0010                 | -0.0133<br>0.0010                | 0.0037<br>0.0010                 | -0.01405<br>0.00097              | 0.0000<br>0.0010                 | -0.0015<br>0.0010                | -0.0002<br>0.0010                | 6369  | 6     | 1957       | 3.9                   | 1.7                    | 1.2                               |
| 015574 | 0.568111 | 6377.86616<br>0.00028        | 17.50792<br>0.00045   | -0.00173<br>0.00066              | 0.10556<br>0.00064               | -0.00402<br>0.00064              | -0.01006<br>0.00064              | 0.00090<br>0.00061               | 0.00000<br>0.00063               | 0.00068<br>0.00064               | -0.00068<br>0.00063              | 4870  | 6     | 2072       | 5.3                   | 1.9                    | 1.4                               |
| 015690 | 0.320057 | 6378.90419<br>0.00056        | 18.8464<br>0.0013     | 0.0005<br>0.0019                 | 0.1140<br>0.0018                 | -0.0002<br>0.0018                | -0.0114<br>0.0018                | 0.0034<br>0.0017                 | 0.0000<br>0.0018                 | -0.0010<br>0.0018                | -0.0005<br>0.0018                | 4877  | 6     | 2072       | 3.6                   | 2.7                    | 1.8                               |
| 015738 | 1.011149 | 3868.82397<br>0.00083        | 14.62047<br>0.00054   | -0.00703<br>0.00077              | 0.10369<br>0.00077               | 0.00088<br>0.00077               | -0.00467<br>0.00076              | 0.00943<br>0.00077               | 0.00000<br>0.00077               | -0.00023<br>0.00077              | -0.00083<br>0.00078              | 731   | 8     | 2617       | 8.2                   | 1.8                    | 1.3                               |
| 015943 | 1.266009 | 6237.24955<br>0.00038        | 16.83388<br>0.00021   | -0.00374<br>0.00031              | 0.11238<br>0.00030               | -0.00542<br>0.00030              | -0.00901<br>0.00030              | 0.00452<br>0.00029               | 0.00000<br>0.00030               | 0.00074<br>0.00030               | -0.00022<br>0.00030              | 4678  | 6     | 2072       | 2.9                   | 2.5                    | 1.7                               |
| 015985 | 0.747424 | 6478.77584<br>0.00051        | 16.70800<br>0.00054   | -0.01884<br>0.00080              | 0.10878<br>0.00078               | -0.00907<br>0.00078              | -0.01231<br>0.00077              | 0.00042<br>0.00075               | 0.00000<br>0.00077               | 0.00692<br>0.00076               | 0.00001<br>0.00077               | 10500 | 6     | 2072       | 42                    | 2.2                    | 1.5                               |
| 016000 | 0.581969 | 6067.49790<br>0.00029        | 15.97686<br>0.00056   | -0.00149<br>0.00080              | 0.12285<br>0.00078               | -0.00577<br>0.00082              | -0.01324<br>0.00081              | 0.00093<br>0.00079               | 0.00000<br>0.00082               | 0.00147<br>0.00078               | 0.00023<br>0.00079               | 590   | 6     | 2040       | 7.3                   | 4.0                    | 2.6                               |
| 016007 | 1.189715 | 6371.5830<br>0.0013          | 18.7220<br>0.0010     | -0.0203<br>0.0016                | 0.1413<br>0.0015                 | -0.0084<br>0.0015                | -0.0196<br>0.0015                | 0.0014<br>0.0014                 | 0.0000<br>0.0015                 | 0.0009<br>0.0015                 | 0.0020<br>0.0015                 | 4803  | 6     | 2072       | 3.2                   | 9.7                    | 5.3                               |
| 016565 | 1.089814 | 6379.62931<br>0.00033        | 16.04945<br>0.00024   | -0.00180<br>0.00035              | 0.11879<br>0.00034               | 0.00220<br>0.00035               | -0.00762<br>0.00034              | -0.00020<br>0.00033              | 0.00000<br>0.00034               | -0.00023<br>0.00033              | -0.00006<br>0.00034              | 1518  | 6     | 2073       | 2.4                   | 3.3                    | 2.2                               |
| 016600 | 0.895531 | 6380.09452<br>0.00021        | 14.82335<br>0.00017   | -0.00567<br>0.00024              | 0.10958<br>0.00024               | 0.00460<br>0.00024               | -0.00852<br>0.00024              | -0.00085<br>0.00024              | 0.00000<br>0.00024               | 0.00020<br>0.00024               | -0.00031<br>0.00024              | 1520  | 6     | 2073       | 2.8                   | 2.3                    | 1.6                               |
| 016749 | 0.502139 | 6378.868309<br>0.000097      | 14.00889<br>0.00016   | -0.00120<br>0.00022              | 0.12029<br>0.00022               | -0.00232<br>0.00022              | -0.00821<br>0.00022              | 0.00032<br>0.00022               | 0.00000<br>0.00022               | 0.00064<br>0.00022               | -0.00026<br>0.00022              | 1518  | 6     | 2073       | 2.4                   | 3.5                    | 2.3                               |
| 016828 | 1.198997 | 6379.89157<br>0.00014        | 13.69730<br>0.00086   | 0.00427<br>0.00012               | 0.11871<br>0.00012               | -0.00444<br>0.00012              | -0.01209<br>0.00012              | 0.01078<br>0.00012               | 0.00000<br>0.00012               | 0.00022<br>0.00012               | -0.00032<br>0.00012              | 4882  | 6     | 2072       | 2.2                   | 3.3                    | 2.2                               |
| 016882 | 0.822556 | 6379.3678<br>0.0012          | 19.0139<br>0.0011     | -0.0116<br>0.0016                | 0.1067<br>0.0015                 | -0.0071<br>0.0015                | -0.0010<br>0.0015                | 0.0010<br>0.0015                 | 0.0000<br>0.0015                 | -0.0005<br>0.0015                | -0.0007<br>0.0015                | 4874  | 6     | 2072       | 2.9                   | 2.0                    | 1.4                               |
| 016961 | 0.460360 | 6218.1901<br>0.0011          | 18.2920<br>0.0014     | -0.0025<br>0.0021                | 0.0975<br>0.0021                 | -0.0053<br>0.0020                | -0.0087<br>0.0021                | 0.0004<br>0.0020                 | 0.0000<br>0.0020                 | -0.0004<br>0.0021                | 0.0021<br>0.0020                 | 1406  | 6     | 2073       | 4.1                   | 1.4                    | 1.0                               |
| 017195 | 0.388208 | 6377.09679<br>0.00065        | 19.0661<br>0.0013     | 0.0014<br>0.0019                 | 0.1082<br>0.0018                 | 0.0039<br>0.0018                 | -0.0048<br>0.0018                | 0.0016<br>0.0017                 | 0.0000<br>0.0018                 | -0.0011<br>0.0018                | 0.0012<br>0.0018                 | 4875  | 6     | 2072       | 3.6                   | 2.1                    | 1.5                               |

Table S1. Continued

| ID     | P        | T <sub>0</sub>         | I                    | a <sub>1c</sub>     | a <sub>2c</sub>     | a <sub>3c</sub>     | a <sub>4c</sub>     | a <sub>1s</sub>     | a <sub>2s</sub>     | a <sub>3s</sub>     | a <sub>4s</sub>     | N     | N <sub>s</sub> | Δt   | χ <sup>2</sup> <sub>red</sub> | q <sub>min</sub> | q <sup>-1σ</sup> <sub>min</sub> |
|--------|----------|------------------------|----------------------|---------------------|---------------------|---------------------|---------------------|---------------------|---------------------|---------------------|---------------------|-------|----------------|------|-------------------------------|------------------|---------------------------------|
|        |          | T <sub>0,err</sub>     | I <sub>err</sub>     | a <sub>1c,err</sub> | a <sub>2c,err</sub> | a <sub>3c,err</sub> | a <sub>4c,err</sub> | a <sub>1s,err</sub> | a <sub>2s,err</sub> | a <sub>3s,err</sub> | a <sub>4s,err</sub> |       |                |      |                               |                  |                                 |
| 017265 | 0.414860 | 6117.53124<br>0.00023  | 15.01804<br>0.00035  | -0.00029<br>0.00050 | 0.09757<br>0.00049  | 0.00235<br>0.00050  | -0.00733<br>0.00049 | 0.00051<br>0.00049  | 0.00000<br>0.00050  | 0.00013<br>0.00048  | 0.00045<br>0.00049  | 646   | 6              | 2069 | 5.1                           | 1.4              | 1.0                             |
| 017836 | 0.819156 | 6479.90724<br>0.00056  | 18.28607<br>0.00056  | -0.01884<br>0.00084 | 0.10685<br>0.00080  | -0.00703<br>0.00079 | 0.00263<br>0.00076  | 0.00378<br>0.00076  | 0.00000<br>0.00080  | 0.00129<br>0.00079  | -0.00100<br>0.00079 | 10524 | 6              | 2072 | 4.5                           | 2.0              | 1.4                             |
| 017953 | 1.338031 | 6379.01268<br>0.00013  | 13.552864<br>0.00093 | -0.00348<br>0.00013 | 0.13763<br>0.00013  | 0.00529<br>0.00013  | -0.01389<br>0.00013 | -0.00037<br>0.00013 | 0.00000<br>0.00013  | 0.00006<br>0.00013  | -0.00014<br>0.00013 | 4873  | 6              | 2072 | 2.6                           | 8.0              | 4.6                             |
| 018058 | 0.248898 | 6378.776160<br>0.00084 | 16.62602<br>0.00031  | -0.02969<br>0.00046 | 0.11143<br>0.00044  | -0.01384<br>0.00044 | 0.00261<br>0.00044  | -0.00528<br>0.00043 | 0.00000<br>0.00044  | 0.00025<br>0.00044  | -0.00053<br>0.00044 | 4883  | 6              | 2072 | 6.7                           | 2.4              | 1.7                             |
| 018179 | 0.499739 | 6377.67900<br>0.00041  | 18.26201<br>0.00064  | -0.0071<br>0.0010   | 0.11003<br>0.00091  | -0.00402<br>0.00089 | -0.00751<br>0.00088 | -0.00273<br>0.00090 | 0.00000<br>0.00090  | -0.00153<br>0.00088 | 0.00070<br>0.00089  | 4874  | 6              | 2072 | 2.9                           | 2.3              | 1.6                             |
| 018395 | 0.387530 | 6217.68312<br>0.00060  | 18.4190<br>0.0014    | -0.0147<br>0.0022   | 0.1460<br>0.0021    | -0.0037<br>0.0020   | -0.0121<br>0.0020   | -0.0102<br>0.0018   | 0.0000<br>0.0020    | 0.0017<br>0.0020    | 0.0006<br>0.0020    | 1403  | 6              | 2073 | 4.4                           | 13               | 6.5                             |
| 018579 | 0.469085 | 6141.89916<br>0.00076  | 18.1811<br>0.0011    | -0.0010<br>0.0017   | 0.1093<br>0.0016    | -0.0049<br>0.0015   | -0.0172<br>0.0016   | 0.0019<br>0.0015    | 0.0000<br>0.0016    | 0.0026<br>0.0016    | -0.0002<br>0.0016   | 1209  | 6              | 2074 | 3.6                           | 2.2              | 1.6                             |
| 018899 | 0.393118 | 6478.78199<br>0.00045  | 18.42993<br>0.00083  | -0.0024<br>0.0012   | 0.1002<br>0.0012    | -0.0021<br>0.0012   | -0.0101<br>0.0012   | -0.0020<br>0.0011   | 0.0000<br>0.0012    | -0.0010<br>0.0012   | 0.0012<br>0.0012    | 10458 | 6              | 2072 | 8.5                           | 1.6              | 1.1                             |
| 019256 | 0.417459 | 6104.80177<br>0.00047  | 18.2391<br>0.0016    | -0.0051<br>0.0024   | 0.1790<br>0.0023    | -0.0017<br>0.0023   | -0.0211<br>0.0022   | 0.0034<br>0.0021    | 0.0000<br>0.0022    | -0.0011<br>0.0022   | -0.0022<br>0.0023   | 1443  | 6              | 2063 | 11                            | 20               | 20                              |
| 019580 | 0.413961 | 6415.97629<br>0.00010  | 15.20552<br>0.00017  | -0.00633<br>0.00025 | 0.11004<br>0.00025  | -0.00401<br>0.00024 | -0.01113<br>0.00025 | 0.00333<br>0.00024  | 0.00000<br>0.00024  | 0.00046<br>0.00025  | -0.00031<br>0.00024 | 4537  | 6              | 1992 | 8.3                           | 2.3              | 1.6                             |
| 019621 | 0.547716 | 6487.75119<br>0.00012  | 17.06406<br>0.00018  | -0.00123<br>0.00026 | 0.12368<br>0.00025  | -0.00351<br>0.00025 | -0.00981<br>0.00025 | 0.00116<br>0.00024  | 0.00000<br>0.00025  | 0.00023<br>0.00025  | 0.00021<br>0.00025  | 10244 | 6              | 2072 | 3.1                           | 4.1              | 2.6                             |
| 019680 | 0.383497 | 6152.85815<br>0.00029  | 16.34445<br>0.00048  | -0.00216<br>0.00067 | 0.10025<br>0.00069  | -0.00306<br>0.00067 | -0.01067<br>0.00068 | 0.00017<br>0.00069  | 0.00000<br>0.00067  | -0.00031<br>0.00070 | -0.00055<br>0.00069 | 621   | 6              | 2064 | 3.0                           | 1.6              | 1.1                             |
| 019753 | 0.398136 | 6086.42921<br>0.00098  | 18.3629<br>0.0018    | -0.0029<br>0.0026   | 0.1037<br>0.0026    | 0.0015<br>0.0026    | -0.0119<br>0.0026   | -0.0020<br>0.0025   | 0.0000<br>0.0026    | -0.0047<br>0.0025   | 0.0008<br>0.0025    | 602   | 6              | 2053 | 3.9                           | 1.8              | 1.3                             |
| 019772 | 0.811458 | 6202.66866<br>0.00023  | 15.83287<br>0.00024  | -0.00081<br>0.00034 | 0.10811<br>0.00033  | -0.00349<br>0.00033 | -0.00934<br>0.00033 | 0.00017<br>0.00033  | 0.00000<br>0.00034  | 0.00077<br>0.00034  | -0.00012<br>0.00034 | 1444  | 6              | 2071 | 2.5                           | 2.1              | 1.5                             |
| 020043 | 0.501081 | 6106.69704<br>0.00080  | 17.2918<br>0.0014    | -0.0037<br>0.0021   | 0.1063<br>0.0020    | -0.0072<br>0.0020   | -0.0062<br>0.0020   | -0.0016<br>0.0019   | 0.0000<br>0.0020    | 0.0002<br>0.0019    | -0.0019<br>0.0019   | 633   | 6              | 2071 | 7.1                           | 2.0              | 1.4                             |

Table S1. Continued

| ID     | $P$      | $T_0$<br>$T_{0, \text{err}}$ | $I$<br>$I_{\text{err}}$ | $a_{1c}$<br>$a_{1c, \text{err}}$ | $a_{2c}$<br>$a_{2c, \text{err}}$ | $a_{3c}$<br>$a_{3c, \text{err}}$ | $a_{4c}$<br>$a_{4c, \text{err}}$ | $a_{1s}$<br>$a_{1s, \text{err}}$ | $a_{2s}$<br>$a_{2s, \text{err}}$ | $a_{3s}$<br>$a_{3s, \text{err}}$ | $a_{4s}$<br>$a_{4s, \text{err}}$ | $N$  | $N_s$ | $\Delta t$ | $\chi^2_{\text{red}}$ | $\hat{q}_{\text{min}}$ | $\hat{q}_{\text{min}}^{-1\sigma}$ |
|--------|----------|------------------------------|-------------------------|----------------------------------|----------------------------------|----------------------------------|----------------------------------|----------------------------------|----------------------------------|----------------------------------|----------------------------------|------|-------|------------|-----------------------|------------------------|-----------------------------------|
| 020168 | 0.778072 | 6200.69299<br>0.00036        | 16.82905<br>0.00035     | 0.00063<br>0.00051               | 0.10491<br>0.00050               | 0.00282<br>0.00050               | -0.00877<br>0.00050              | 0.00118<br>0.00047               | 0.00000<br>0.00048               | -0.00068<br>0.00049              | -0.00026<br>0.00048              | 1541 | 6     | 2069       | 3.2                   | 1.9                    | 1.3                               |
| 020383 | 0.598181 | 6338.38439<br>0.00064        | 17.56153<br>0.00089     | -0.00015<br>0.00013              | 0.0993<br>0.0013                 | -0.0021<br>0.0013                | -0.0060<br>0.0013                | 0.0004<br>0.0012                 | 0.0000<br>0.0013                 | -0.0000<br>0.0013                | -0.0005<br>0.0013                | 1486 | 6     | 2071       | 3.9                   | 1.5                    | 1.1                               |
| 020508 | 0.533814 | 6341.41407<br>0.00079        | 17.9880<br>0.0013       | -0.00016<br>0.00019              | 0.1009<br>0.0018                 | -0.0029<br>0.0019                | -0.0059<br>0.0018                | -0.0014<br>0.0017                | 0.0000<br>0.0018                 | -0.0017<br>0.0018                | 0.0017<br>0.0018                 | 1490 | 6     | 2071       | 4.2                   | 1.6                    | 1.1                               |
| 020763 | 0.710296 | 6124.77341<br>0.00043        | 16.47438<br>0.00039     | -0.00567<br>0.00056              | 0.10159<br>0.00055               | 0.00324<br>0.00054               | -0.00797<br>0.00056              | -0.00303<br>0.00053              | 0.00000<br>0.00054               | -0.00060<br>0.00055              | 0.00016<br>0.00054               | 960  | 6     | 2011       | 4.0                   | 1.6                    | 1.2                               |
| 020858 | 0.412704 | 6104.86352<br>0.00086        | 18.2531<br>0.0016       | -0.0089<br>0.0024                | 0.1089<br>0.0022                 | -0.0049<br>0.0023                | -0.0071<br>0.0023                | 0.0076<br>0.0021                 | 0.0000<br>0.0023                 | -0.0030<br>0.0022                | -0.0016<br>0.0022                | 633  | 6     | 2071       | 2.2                   | 2.2                    | 1.5                               |
| 021027 | 0.760713 | 6370.96434<br>0.00034        | 16.72400<br>0.00035     | -0.00215<br>0.00051              | 0.10060<br>0.00051               | -0.00344<br>0.00049              | -0.00839<br>0.00050              | 0.00285<br>0.00048               | 0.00000<br>0.00049               | 0.00066<br>0.00050               | -0.00048<br>0.00050              | 1505 | 6     | 2071       | 2.3                   | 1.6                    | 1.1                               |
| 021280 | 0.325031 | 6370.33560<br>0.00037        | 17.61797<br>0.00075     | -0.0154<br>0.0011                | 0.0982<br>0.0011                 | -0.0007<br>0.0011                | -0.0075<br>0.0011                | -0.0033<br>0.0010                | 0.0000<br>0.0011                 | 0.0000<br>0.0011                 | 0.0027<br>0.0011                 | 1454 | 6     | 2069       | 4.3                   | 1.4                    | 1.0                               |
| 021400 | 0.680623 | 6195.81706<br>0.00028        | 15.95894<br>0.00030     | -0.00652<br>0.00043              | 0.10830<br>0.00042               | 0.00367<br>0.00041               | -0.00783<br>0.00042              | 0.00073<br>0.00042               | 0.00000<br>0.00042               | -0.00081<br>0.00043              | 0.00009<br>0.00042               | 981  | 6     | 2058       | 2.6                   | 2.2                    | 1.5                               |
| 021449 | 0.716299 | 6183.83087<br>0.00046        | 16.99018<br>0.00046     | -0.00326<br>0.00067              | 0.10104<br>0.00065               | 0.00444<br>0.00066               | -0.00605<br>0.00066              | -0.00148<br>0.00063              | 0.00000<br>0.00065               | -0.00001<br>0.00065              | -0.00031<br>0.00065              | 1282 | 6     | 2071       | 4.5                   | 1.6                    | 1.2                               |
| 021677 | 0.365884 | 6371.48000<br>0.00066        | 18.4516<br>0.0014       | -0.0224<br>0.0021                | 0.1130<br>0.0021                 | -0.0093<br>0.0020                | -0.0080<br>0.0020                | 0.0229<br>0.0019                 | 0.0000<br>0.0020                 | -0.0012<br>0.0020                | -0.0010<br>0.0021                | 1508 | 6     | 2071       | 5.9                   | 2.6                    | 1.8                               |
| 021877 | 0.442422 | 6343.78414<br>0.00016        | 15.04932<br>0.00025     | -0.00150<br>0.00036              | 0.10053<br>0.00035               | -0.00254<br>0.00035              | -0.00557<br>0.00035              | -0.00070<br>0.00035              | 0.00000<br>0.00036               | 0.00027<br>0.00036               | -0.00026<br>0.00036              | 1492 | 6     | 2071       | 6.1                   | 1.6                    | 1.1                               |
| 022020 | 0.453845 | 6191.40535<br>0.00080        | 18.1267<br>0.0015       | -0.0052<br>0.0022                | 0.1196<br>0.0021                 | -0.0060<br>0.0020                | -0.0075<br>0.0021                | 0.0033<br>0.0020                 | 0.0000<br>0.0021                 | 0.0031<br>0.0021                 | 0.0002<br>0.0021                 | 1376 | 6     | 2071       | 4.8                   | 3.4                    | 2.3                               |
| 022024 | 0.486984 | 6158.6675<br>0.0016          | 17.9937<br>0.0021       | -0.0312<br>0.0031                | 0.0999<br>0.0031                 | -0.0113<br>0.0030                | -0.0055<br>0.0030                | -0.0011<br>0.0028                | 0.0000<br>0.0029                 | -0.0020<br>0.0030                | 0.0008<br>0.0030                 | 768  | 6     | 2070       | 9.7                   | 1.5                    | 1.1                               |
| 022106 | 0.784120 | 6387.19651<br>0.00028        | 16.03855<br>0.00025     | -0.00275<br>0.00037              | 0.11050<br>0.00036               | 0.00497<br>0.00036               | -0.01191<br>0.00036              | -0.00220<br>0.00035              | 0.00000<br>0.00036               | -0.00047<br>0.00036              | 0.00018<br>0.00036               | 1451 | 6     | 2071       | 2.7                   | 2.4                    | 1.6                               |
| 022365 | 0.428554 | 6125.06643<br>0.00091        | 17.9287<br>0.0015       | -0.0058<br>0.0022                | 0.1069<br>0.0022                 | 0.0035<br>0.0021                 | -0.0099<br>0.0021                | 0.0091<br>0.0020                 | 0.0000<br>0.0021                 | -0.0013<br>0.0021                | 0.0001<br>0.0022                 | 492  | 6     | 2059       | 3.8                   | 2.0                    | 1.4                               |

Table S1. Continued

| ID     | P        | $T_0$              | I                | $a_{1c}$            | $a_{2c}$            | $a_{3c}$            | $a_{4c}$            | $a_{1s}$            | $a_{2s}$            | $a_{3s}$            | $a_{4s}$            | N   | $N_s$ | $\Delta t$ | $\chi^2_{\text{red}}$ | $\hat{q}_{\text{min}}$ | $\hat{q}_{\text{min}}^{-1\sigma}$ |
|--------|----------|--------------------|------------------|---------------------|---------------------|---------------------|---------------------|---------------------|---------------------|---------------------|---------------------|-----|-------|------------|-----------------------|------------------------|-----------------------------------|
|        |          | $T_{0,\text{err}}$ | $I_{\text{err}}$ | $a_{1c,\text{err}}$ | $a_{2c,\text{err}}$ | $a_{3c,\text{err}}$ | $a_{4c,\text{err}}$ | $a_{1s,\text{err}}$ | $a_{2s,\text{err}}$ | $a_{3s,\text{err}}$ | $a_{4s,\text{err}}$ |     |       |            |                       |                        |                                   |
| 022852 | 0.807296 | 6380.9601          | 17.5582          | -0.0130             | 0.1342              | -0.0076             | -0.0149             | -0.0007             | 0.0000              | -0.0032             | -0.0013             | 339 | 6     | 2071       | 15                    | 6.7                    | 3.9                               |
|        |          | 0.0022             | 0.0023           | 0.0037              | 0.0035              | 0.0034              | 0.0034              | 0.0031              | 0.0034              | 0.0034              | 0.0033              |     |       |            |                       |                        |                                   |
| 022976 | 0.607784 | 6122.20134         | 16.59065         | -0.00172            | 0.10698             | -0.00203            | -0.00686            | 0.00039             | 0.00000             | -0.00041            | 0.00129             | 651 | 6     | 2071       | 3.2                   | 2.0                    | 1.4                               |
|        |          | 0.00041            | 0.00055          | 0.00081             | 0.00078             | 0.00076             | 0.00078             | 0.00075             | 0.00078             | 0.00080             | 0.00078             |     |       |            |                       |                        |                                   |
| 022996 | 0.917919 | 6402.81730         | 16.63786         | 0.00453             | 0.10372             | -0.00304            | -0.00774            | 0.00511             | 0.00000             | 0.00152             | 0.00060             | 328 | 6     | 2072       | 1.6                   | 1.8                    | 1.3                               |
|        |          | 0.00082            | 0.00066          | 0.00100             | 0.00098             | 0.00092             | 0.00094             | 0.00091             | 0.00093             | 0.00099             | 0.00097             |     |       |            |                       |                        |                                   |
| 023064 | 1.237897 | 6070.58540         | 15.87145         | -0.01891            | 0.09767             | -0.00540            | -0.01067            | -0.00145            | 0.00000             | -0.00021            | -0.00093            | 471 | 6     | 2016       | 3.0                   | 1.4                    | 1.0                               |
|        |          | 0.00081            | 0.00050          | 0.00073             | 0.00069             | 0.00071             | 0.00069             | 0.00070             | 0.00074             | 0.00071             | 0.00073             |     |       |            |                       |                        |                                   |
| 023746 | 0.506929 | 6115.27650         | 17.29144         | -0.0003             | 0.1004              | -0.0030             | -0.0055             | 0.0024              | 0.0000              | -0.0005             | -0.0006             | 640 | 6     | 2071       | 2.7                   | 1.6                    | 1.1                               |
|        |          | 0.00058            | 0.00078          | 0.0012              | 0.0011              | 0.0011              | 0.0011              | 0.0011              | 0.0011              | 0.0011              | 0.0011              |     |       |            |                       |                        |                                   |
| 023863 | 0.695058 | 6118.44368         | 15.38107         | -0.00216            | 0.10109             | 0.00461             | -0.00773            | -0.00114            | 0.00000             | 0.00012             | 0.00086             | 650 | 6     | 2070       | 3.0                   | 1.6                    | 1.2                               |
|        |          | 0.00034            | 0.00031          | 0.00047             | 0.00045             | 0.00044             | 0.00044             | 0.00043             | 0.00045             | 0.00045             | 0.00045             |     |       |            |                       |                        |                                   |
| 023906 | 1.284907 | 6205.55179         | 15.41725         | 0.00759             | 0.09957             | -0.00227            | -0.00746            | 0.01021             | 0.00000             | 0.00044             | -0.00023            | 367 | 6     | 2068       | 1.9                   | 1.5                    | 1.1                               |
|        |          | 0.00074            | 0.00043          | 0.00063             | 0.00061             | 0.00063             | 0.00062             | 0.00060             | 0.00062             | 0.00061             | 0.00061             |     |       |            |                       |                        |                                   |
| 024048 | 0.772261 | 6069.93919         | 15.79633         | -0.00811            | 0.10391             | 0.00273             | -0.00618            | 0.00059             | 0.00000             | -0.00023            | -0.00075            | 587 | 6     | 2059       | 13                    | 1.8                    | 1.3                               |
|        |          | 0.00053            | 0.00047          | 0.00069             | 0.00067             | 0.00067             | 0.00069             | 0.00065             | 0.00066             | 0.00066             | 0.00065             |     |       |            |                       |                        |                                   |
| 024067 | 0.877599 | 6201.48950         | 15.63023         | 0.00204             | 0.10154             | -0.00449            | -0.01060            | 0.00336             | 0.00000             | -0.00001            | -0.00030            | 420 | 6     | 2071       | 1.8                   | 1.6                    | 1.2                               |
|        |          | 0.00038            | 0.00035          | 0.00052             | 0.00051             | 0.00051             | 0.00050             | 0.00048             | 0.00049             | 0.00050             | 0.00050             |     |       |            |                       |                        |                                   |
| 024347 | 0.889661 | 6182.29120         | 15.41972         | -0.00743            | 0.10332             | 0.00356             | -0.00700            | -0.00096            | 0.00000             | 0.00043             | -0.00067            | 365 | 6     | 2070       | 1.6                   | 1.8                    | 1.3                               |
|        |          | 0.00048            | 0.00035          | 0.00052             | 0.00051             | 0.00050             | 0.00051             | 0.00047             | 0.00050             | 0.00050             | 0.00049             |     |       |            |                       |                        |                                   |
| 024378 | 0.599922 | 6023.20600         | 13.37639         | -0.0044             | 0.1027              | 0.0019              | -0.0116             | 0.0002              | 0.0000              | 0.0027              | 0.00014             | 194 | 4     | 1323       | 6.6                   | 1.7                    | 1.2                               |
|        |          | 0.00064            | 0.00072          | 0.0010              | 0.0010              | 0.0010              | 0.0011              | 0.0010              | 0.0011              | 0.0010              | 0.00097             |     |       |            |                       |                        |                                   |
| 024463 | 1.108817 | 6209.07644         | 15.67801         | -0.00071            | 0.09985             | -0.00502            | -0.00835            | 0.00361             | 0.00000             | 0.00007             | 0.00051             | 368 | 6     | 2068       | 1.7                   | 1.5                    | 1.1                               |
|        |          | 0.00068            | 0.00039          | 0.00055             | 0.00054             | 0.00055             | 0.00056             | 0.00055             | 0.00056             | 0.00055             | 0.00055             |     |       |            |                       |                        |                                   |
| 024562 | 0.760747 | 6191.18842         | 16.40300         | -0.0057             | 0.1092              | 0.0018              | -0.0079             | -0.0013             | 0.0000              | -0.0003             | -0.0011             | 364 | 6     | 2068       | 5.0                   | 2.2                    | 1.5                               |
|        |          | 0.00060            | 0.00073          | 0.0011              | 0.0010              | 0.0010              | 0.0010              | 0.0010              | 0.0011              | 0.0011              | 0.0011              |     |       |            |                       |                        |                                   |
| 024717 | 0.962187 | 6172.86556         | 15.72430         | -0.00494            | 0.11866             | 0.00270             | -0.00766            | 0.00045             | 0.00000             | -0.00061            | 0.00093             | 411 | 6     | 2072       | 4.4                   | 3.3                    | 2.2                               |
|        |          | 0.00042            | 0.00043          | 0.00064             | 0.00063             | 0.00064             | 0.00061             | 0.00060             | 0.00062             | 0.00060             | 0.00063             |     |       |            |                       |                        |                                   |
| 024866 | 0.994403 | 6123.11015         | 14.61658         | 0.00030             | 0.09785             | -0.00593            | -0.00891            | 0.00298             | 0.00000             | 0.00019             | -0.00014            | 380 | 6     | 2071       | 1.7                   | 1.4                    | 1.0                               |
|        |          | 0.00036            | 0.00029          | 0.00042             | 0.00040             | 0.00042             | 0.00040             | 0.00043             | 0.00043             | 0.00040             | 0.00042             |     |       |            |                       |                        |                                   |
| 025039 | 0.889109 | 6173.31605         | 15.74399         | -0.00860            | 0.09769             | 0.00177             | -0.00619            | 0.00086             | 0.00000             | 0.00022             | 0.00079             | 363 | 6     | 2070       | 3.7                   | 1.4                    | 1.0                               |
|        |          | 0.00056            | 0.00047          | 0.00071             | 0.00068             | 0.00067             | 0.00067             | 0.00065             | 0.00068             | 0.00068             | 0.00069             |     |       |            |                       |                        |                                   |

Table S1. Continued
